# Supplementary material for: Governing Governance: A Formal Framework for Analysing Institutional Design and Enactment Governance
Source: arXiv:1704.06654 source file (2017-04-21)
Supplement: Supplementary file 1 [file appendices.tex]

\chapter*{Appendices}

{\color{tck-grey}These appendices accompany the dissertation titled Governing Governance: A Formal Framework for Analysing Institutional Design and Enactment Governance by Thomas C. King - Technical University of Delft}

\newpage

\section{Multi-Level Governance Computational Framework Proofs}
\label{secAppCompProofs}

\subsection{Deontological Counts-as Soundness Proof}
\label{proofAbstraction}
\begin{proof}{Lemma~\ref{theoremAbstraction}} We need to show that $S^{i}_{j} \subseteq \overline{\textit{DC}}^{i}(S^{i}_{j})$ and $\overline{\textit{DC}}^{i}(S^{i}_{j}) \subseteq S^{i}_{j}$. Each case is dealt with separately:
\begin{enumerate}
\item $S^{i}_{j} \subseteq \overline{\textit{DC}}^{i}(S^{i}_{j})$ - If $f \in S^{i}_{j}$ then $f \in \overline{\textit{DC}}^{i}(S^{i}_{j})$ due to monotonicity of $\overline{\textit{DC}}^{i}$.
\item $\overline{\textit{DC}}^{i}(S^{i}_{j}) \subseteq S^{i}_{j}$ - given that if $\langle N, n \rangle \in \textit{DC}(S^{i}_{j})$ and $S^{i}_{j} \models N$ then $n \in \overline{\textit{DC}}^{i}(S^{i}_{j})$, we need to show that $n \in S^{i}_{j}$. By construction of $S^{i}_{j}$ we know that $n \in S^{i}_{j}$ iff $M_{P} \models \asp{holdsat(} n, \textit{In}^{i}, j)$, in turn we know $M_{P} \models \asp{holdsat(} n, \textit{In}^{i}, j)$ iff $\asp{holdsat(} n, \textit{In}^{i}, j)$ is an atom in the head of an applied rule. We show for every $\langle N, n \rangle \in \textit{DC}(S^{i}_{j})$ and $n$ given in Definition~\ref{defDC}, under the assumption that $S^{i}_{j} \models N$ that there is an applied rule $r$ with the atom $\asp{holdsat(} n, \textit{In}^{i}, j) = H(r)$ in the head. By induction on two counters:
\begin{enumerate}[label*=\arabic*.]
\item \label{proofDCBCaseObl} \textbf{Base case 1:} According to \ref{eqDC1} $N = \{ \textit{obl}(a, d) \}$ and $n = \textit{obl}(b, d)$ where $b \in \pazocal{E}^{i} \cup \pazocal{F}^{i}$. From \ref{eqDC1} we know that $\exists a \in \pazocal{E}^{i} \pazocal{F}^{i}$ and $\exists X \in \pazocal{X}^{i}$ s.t. $S^{i}_{j} \models X$ and $b \in \pazocal{G}^{i}(X, a) \cup \pazocal{D}^{i}(X, a)$, and $n \in \pazocal{F}^{i}_{\textit{anorm}}$. Thus, the conditions on the left hand side of transformation \ref{eqASPDCATrans1} or are met and therefore we have an AnsProlog rule $\asp{holdsat(obl(}b, d\asp{)}, \textit{In}^i, I \asp{) :- }$ \\$\textit{CN}\asp{,} \textit{C} \asp{,} \asp{holdsat(pow(}b\asp{),} \textit{In}^{i}, I\asp{),} \asp{nifluent(}\textit{obl(}b, d\asp{)}, \textit{In}^{i} \asp{),} \asp{instant(I).}$ or the conditions of transformation \ref{eqASPDCATrans5} are met and we have an AnsProlog rule \\$\asp{holdsat(obl(}b, d\asp{)}, \textit{In}^i, I \asp{) :- }
\textit{CN}\asp{,} \textit{C} \asp{,} \asp{nifluent(}\textit{obl(}b, d\asp{)}, \textit{In}^{i} \asp{),} \asp{instant(I).}$. Since according to \ref{eqASPSemTrans16} \\$\asp{instant(}j\asp{).} \in \Pi^{\textit{base(k)}}$ is a fact, therefore $M_{P} \models \asp{instant(}j\asp{)}$ and we have a ground rule $r = \asp{holdsat(obl(}b, d\asp{)}, \textit{In}^i, j \asp{) :- }$ \\$
\textit{CN}\asp{,} \textit{C} \asp{,} \asp{holdsat(pow(}b\asp{),} \textit{In}^{i}, j\asp{),} \asp{nifluent(}\textit{obl(}b, d\asp{)}, \textit{In}^{i} \asp{),} \asp{instant(}j\asp{).} \in P^{*}$ or a ground rule $r = \asp{holdsat(obl(}b, d\asp{)}, \textit{In}^i, j \asp{) :- }$ \\$
\textit{CN}\asp{,} \textit{C} \asp{,} \asp{nifluent(}\textit{obl(}b, d\asp{)}, \textit{In}^{i} \asp{),} \asp{instant(}j\asp{).} \in P^{*}$ where \\ $\textit{CN} = \{\textit{EX(obl(a, d),} \pazocal{I}^{i}) \asp{:} \textit{EX(X}^{i}, \pazocal{I}^{i})\asp{;}\}$ and $C = \asp{1\{} \textit{CN} \asp{\}}$. We need to show \\$\forall l \in B(r) : M_P \models l$:
\begin{enumerate}[label*=\arabic*.]
\item $\textit{CN}$ - According to \ref{eqASPDCATrans1} $\textit{CN} = \{\textit{EX(obl(a, d),} \pazocal{I}^{i}) \asp{:} \textit{EX(X}, \pazocal{I}^{i})\asp{;}\}$ is a singleton containing a conditional literal and according to Definition~\ref{defASPDCATrans} \\$\textit{EX(obl(a, d),} \pazocal{I}^{i}) \asp{:} \textit{EX(X}^{i}, \pazocal{I}^{i})\asp{;} \in B(r)$. We will show that if $M_P \models \textit{EX(X}^{i}, \pazocal{I}^{i})\asp{;}$ then assuming $S^{i}_{j} \models N$ that $M_P \models \textit{EX(obl(a, d),} \pazocal{I}^{i})$:
\begin{enumerate}[label*=\arabic*.]
\item By \ref{eqASPDCATrans1} or \ref{eqASPDCATrans5} $\textit{CN}$ is constructed such that if \\$\textit{EX(obl(a,d), } \pazocal{I}^{i}) \asp{:} \textit{EX(X, } \pazocal{I}^{i})\asp{;} \in \textit{CN}$ then $a \in \pazocal{E}^{i} \cap \pazocal{F}^{i}, X \in \pazocal{X}^{i}$ s.t. $b \in \pazocal{G}^{i}(X, a) \cap \pazocal{D}^{i}(X, $.
\item If $X = \emptyset$ then $\textit{EX(X, } \pazocal{I}^{i})$ translates to $\asp{\#true}$ and it is always the case that $M_P \models \asp{\#true}$ and since $X = \emptyset$ we have $S^{i}_{j} \models X$.
\item If $X \neq \emptyset$ and $M_P \models \textit{EX(X, } \pazocal{I}^{i})$ then since $\textit{EX(X, } \pazocal{I}^{i})$ translates to \\$\asp{holdsat}/3$ literals, by construction of $S^{i}_{j}$ it is the case that $S^{i}_{j} \models X$. 
\item By $N$ we have $N = \{ \textit{obl}(a,d)\}$ and assuming $S^{i}_{j} \models N$ we have $S^{i}_{j} \models \textit{obl}(a,d)$ and by construction of $S^{i}_{j}$ we have $M_P \models \textit{EX(obl(a,d), } \pazocal{I}^{i})$.
\item By 2.1.1.1., 2.1.2. and 2.1.1.3. and construction and construction of $S^{i}_{j}$ we have $M_P \models \textit{EX(X}^{i}, \pazocal{I}^{i})\asp{;}$ and with 2.1.1.4 we have $M_P \models \textit{EX(obl(a,d), } \pazocal{I}^{i}) \asp{:} \textit{EX(X, } \pazocal{I}^{i})$.
\end{enumerate}
We have shown that for all $\textit{EX(obl(a,d), } \pazocal{I}^{i}) \asp{:} \textit{EX(X, } \pazocal{I}^{i})\asp{;}$ in $\textit{CN} : M_P \models \textit{EX(X, } \pazocal{I}^{i})$ it is the case that  $\textit{obl}(a,d) \in N$ and therefore that $M_P \models \textit{EX(obl(a,d), } \pazocal{I}^{i})$, and $M_P \models \textit{CN}$.
\item $C$ - According to \ref{eqASPDCATrans1} $C = \asp{1\{} \textit{CN} \asp{\}}$, by translation \\$C = \asp{1\{} \asp{holdsat(obl(a, d),} \pazocal{I}^{i}, \asp{I)} : \textit{EX(X}^{i}, \pazocal{I}^{i}) \asp{;\}}$. $C$ is true if at least one element is true, under the semantics of aggregates we need to show $M_P \models \textit{EX(obl(a, d)}, \pazocal{I}^{i})$ and $M_P \models \textit{EX(X}, \pazocal{I}^{i})$.
\begin{enumerate}[label*=\arabic*.]
\item We have already established that $N$ is constructed s.t. $X \in \pazocal{X}^{i}$ and $S^{i}_{j} \models X$. By construction of $S^{i}_{j}$ we have $M_P \models \textit{EX(X}^{i}, \pazocal{I}^{i})$. 
\item Since $\asp{holdsat(obl(a, d),} \pazocal{I}^{i}, \asp{I)} : \textit{EX(X}^{i}, \pazocal{I}^{i}) \asp{;} \in \textit{CN}$ by 2.1.2.1 and 2.1.1.5 we have \\$M_P \models \asp{holdsat(obl(a, d),} \pazocal{I}^{i}, \asp{I)}$.
\end{enumerate}
By 2.1.2.1 and 2.1.2.2 we have $M_P \models C$.
\item In the case that $r$ is produced by \ref{eqASPDCATrans1}  $\asp{holdsat(pow(}b\asp{),} \textit{In}^{i}, j\asp{)}$ - since $N=\{ \textit{obl(a,d)} \}$ the condition of its construction $S^{i}_{j} \models \textit{pow}(b)$ according to \ref{eqDC1} holds. By construction of $S^{i}_{j}$ we know $M_{P} \models \asp{holdsat(pow(}b\asp{),} \textit{In}^{i}, j\asp{)}$.
\item $\asp{nifluent(}\textit{obl(}b, d\asp{)}, \textit{In}^{i})$ - true by $\textit{obl(}b, d\asp{)} \in \pazocal{F}_{\textit{anorm}}$ and \ref{eqASPMLTrans4}.
\item $\asp{instant(}j\asp{)}$ - According to \ref{eqASPSemTrans16} $\asp{instant(}j\asp{).} \in \Pi^{\textit{base(k)}}$ is a fact and therefore $M_{P} \models \asp{instant(}j\asp{)}$.
\end{enumerate}
We have shown that for any $\langle N, n \rangle \in \textit{DC}(S^{i}_{j})$ where $N = \{ \textit{obl}(a, d) \}$ and $n = \textit{obl}(b, d)$ where $b \in \pazocal{E}$ that we have a ground rule \\$r = \asp{holdsat(obl(}b, d\asp{)}, \textit{In}^i, j \asp{) :- }
\textit{CN}\asp{,} \textit{C} \asp{,}\\ \asp{holdsat(pow(}b\asp{),} \textit{In}^{i}, j\asp{),} \asp{instant(}j\asp{).} \in P^{*}$ or a ground rule \\ $r = \asp{holdsat(obl(}b, d\asp{)}, \textit{In}^i, j \asp{) :- } \textit{CN}\asp{,} \textit{C} \asp{,}\\ \asp{instant(}j\asp{).} \in P^{*}$ and that assuming $S^{i}_{j} \models N$ then $\forall l \in B(r) : M_P \models l$ and thus $M_P \models H(r)$ and by construction $S^{i}_{j} \models n$.
\item \label{proofDCBCasePro} \textbf{Base case 2:} According to \ref{eqDC2} $N = \{ \textit{pro}(a_{0}, d), ..., \textit{pro}(a_{l}, d) \}$ and $n = \textit{pro}(b, d)$ where $b \in \pazocal{E}$. We know that from Definition~\ref{defDC} $N \neq \emptyset$ and from \ref{eqDC1} $N$ is constructed as $N = \{ \textit{pro}(a, d) \mid \; \exists X, a : X \in \pazocal{X}^{i} \wedge a \in \pazocal{E}_{\textit{inst}}^{i} \wedge n^{\prime} = \textit{pro}(b, d) \wedge S^{i}_{j} \models X \wedge  b \in \pazocal{G}^{i}(X, a) \wedge S^{i}_{j} \models \textit{pow}(b) \}$ thus on the left hand side of the transformations \ref{eqASPDCATrans2} and \ref{eqASPDCATrans6} the set $\textit{CN}$ is non-empty and since $n \in \pazocal{F}^{i}_{\textit{anorm}}$ all conditions of \ref{eqASPDCATrans2} or \ref{eqASPDCATrans6} are met. Therefore we have an AnsProlog rule $\asp{holdsat(pro(}b, d\asp{)}, \textit{In}^i, I \asp{) :- }$ \\
$\textit{CN}\asp{,} \textit{C} \asp{,} \asp{holdsat(pow(}b\asp{),} \textit{In}^{i}, I\asp{),} \asp{nifluent(}\textit{pro(}b, d\asp{),} \asp{instant(}I\asp{).}$ or an AnsProlog rule $\asp{holdsat(pro(}b, d\asp{)}, \textit{In}^i, I \asp{) :- }$ \\ $\textit{CN}\asp{,} \textit{C} \asp{,} \asp{nifluent(}\textit{pro(}b, d\asp{),} \asp{instant(}I\asp{).}$ and since according to \ref{eqASPSemTrans16} $\asp{instant(}j\asp{).} \in \Pi^{\textit{base(k)}}$ is a fact, we have $M_{P} \models \asp{instant(}j\asp{)}$ and a ground rule \\$r = \asp{holdsat(pro(}b, d\asp{)}, \textit{In}^i, j \asp{) :- }$ \\
$\textit{CN}\asp{,} \textit{C} \asp{,} \asp{holdsat(pow(}b\asp{),} \textit{In}^{i}, j\asp{),} \asp{nifluent(}\textit{pro(}b, d\asp{),} \asp{instant(}j\asp{).} \in P^{*}$ or a ground rule \\ $r = \asp{holdsat(pro(}b, d\asp{)}, \textit{In}^i, j \asp{) :- }
\textit{CN}\asp{,} \textit{C} \asp{,} \asp{nifluent(}\textit{pro(}b, d\asp{),} \asp{instant(}j\asp{).} \in P^{*}$. We need to show each term in the body of $r$ is true in $M_{P}$ s.t. $\forall l \in B(r) : M_{P} \models l$:
\begin{enumerate}[label*=\arabic*.]
\item \textit{CN} - According to \ref{eqASPDCATrans2} or \ref{eqASPDCATrans6} $\textit{CN} = \{ \textit{EX(pro(a,d), } \pazocal{I}^{i}) \asp{:} \textit{EX(X, } \pazocal{I}^{i})\asp{;} \mid a \in \pazocal{E}^{i} \cap \pazocal{F}^{i}, X \in \pazocal{X}^{i}, b \in \pazocal{G}^{i}(X, a) \cap \pazocal{D}^{i}(X, a) \}$ is a set of conditional literals comma-delimited in the rule $r$ according to definition~\ref{defASPDCATrans} s.t. \\$\forall \textit{EX(pro(a,d), } \pazocal{I}^{i}) \asp{:} \textit{EX(X, } \pazocal{I}^{i})\asp{;} \in \textit{CN} : \textit{EX(pro(a,d), } \pazocal{I}^{i}) \asp{:} \textit{EX(X, } \pazocal{I}^{i})\asp{;} \in B(r)$. \\ We will show every conditional literal in $\textit{CN}$ is true s.t. \\$\forall  \textit{EX(pro(a,d), } \pazocal{I}^{i}) \asp{:} \textit{EX(X, } \pazocal{I}^{i})\asp{;} \in \textit{CN}$ if $M_P \models \textit{EX(X, } \pazocal{I}^{i})$ then assuming $S^{i}_{j} \models N$ that $M_P \models \textit{EX(pro(a,d), } \pazocal{I}^{i})$.
\begin{enumerate}[label*=\arabic*.]
\item By \ref{eqASPDCATrans2} or \ref{eqASPDCATrans6} $\textit{CN}$ is constructed such that if $\textit{EX(pro(a,d), } \pazocal{I}^{i}) \asp{:} \textit{EX(X, } \pazocal{I}^{i})\asp{;}$ \\ $\in \textit{CN}$ then $a \in \pazocal{E}^{i} \cap \pazocal{F}^{i}, X \in \pazocal{X}^{i}$ s.t. $b \in \pazocal{G}^{i}(X, a) \cap \pazocal{D}^{i}(X, a)$. 
\item If $X = \emptyset$ then $\textit{EX(X, } \pazocal{I}^{i})$ translates to $\asp{\#true}$ for which it is always the case $M_P \models \asp{\#true}$ and since $X = \emptyset$ we have $S^{i}_{j} \models X$. 
\item If $X \neq \emptyset$ and $M_P \models \textit{EX(X, } \pazocal{I}^{i})$ then since $\textit{EX(X, } \pazocal{I}^{i})$ translates to \\$\asp{holdsat}/3$ literals, by construction of $S^{i}_{j}$ it is the case that $S^{i}_{j} \models X$. 
\item If $M_P \models \textit{EX(X, } \pazocal{I}^{i})$ with 2.1.1. we have $b \in \pazocal{G}^{i}(X, a)$ and by By 2.1.2 and 2.1.3. we have $S^{i}_{j} \models X$ therefore by construction of $N$ we have $\textit{pro}(a,d) \in N$. 
\item Under the assumption that $S^{i}_{j} \models N$, $\textit{pro}(a,d) \in S^{i}_{j}$ and therefore by construction of $S^{i}_{j}$ we have $M_P \models \textit{EX(pro(a,d), } \pazocal{I}^{i})$. 
\item By 2.1.2., 2.1.3 and 2.1.4. by construction of $S^{i}_{j}$ we have $M_P \models \textit{EX(pro(a,d), } \pazocal{I}^{i})$ \\ $\asp{:} \textit{EX(X, } \pazocal{I}^{i})$.
\end{enumerate}
We have shown that for all $\textit{EX(pro(a,d), } \pazocal{I}^{i}) \asp{:} \textit{EX(X, } \pazocal{I}^{i})\asp{;}$ in $\textit{CN}$ if$M_P \models \textit{EX(X, } \pazocal{I}^{i})$  then \\$M_P \models \textit{EX(pro(a,d), } \pazocal{I}^{i})$, and $M_P \models \textit{CN}$.
\item $C$ - According to \ref{eqASPDCATrans2} or \ref{eqASPDCATrans6} $C = \asp{1\{} \textit{CN} \asp{\}}$, is an aggregate which is true if at least one element is true, under the semantics of aggregates we need to show $\exists \textit{EX(pro(a,d), } \pazocal{I}^{i}) \asp{:} \textit{EX(X, } \pazocal{I}^{i})\asp{;} \in \textit{CN} : M_P \models \textit{EX(pro(a, d)}, \pazocal{I}^{i}) \wedge M_P \models \textit{EX(X, } \pazocal{I}^{i})$. 
\begin{enumerate}[label*=\arabic*.]
\item By Definition~\ref{defDC} $N \neq \emptyset$ and by \ref{eqDC2} $N$ is constructed as  $\{ \textit{pro}(a, d) \mid \; \langle A, b \rangle \in \pazocal{A}^{i}(S^{i}) \wedge a \in A \}$ and if by \ref{eqCA1} $\langle A, b \rangle \in \pazocal{A}^{i}(S^{i})$ then $S \models \textit{pow}(b) $. Therefore we know that by \ref{eqCA1} or \ref{eqCA2} $\exists X, a : X \in \pazocal{X}^{i} \wedge a \in \pazocal{E}^{i} \cap \pazocal{F}^{i} \wedge S \models X \wedge  b \in \pazocal{G}^{i}(X, a) \cap \pazocal{D}^{i}(X, a)$.
\item By 2.2.2.1. we have $\textit{pro}(a,d) \in N$ and by construction of $\textit{CN}$ in \ref{eqASPDCATrans2} we have that there exists $\textit{EX(pro(a,d), } \pazocal{I}^{i}) \asp{:} \textit{EX(X, } \pazocal{I}^{i})\asp{;} \in \textit{CN}$ such that $S^{i}_{j} \models X$.
\item By construction of $S^{i}_{j}$ we have $M_P \models \textit{EX(X, } \pazocal{I}^{i})$. 
\item Assuming $S^{i}_{j} \models N$, by 2.2.2.1. and by construction of $S^{i}_{j}$ we have $M_P \models \textit{EX(pro(a,d), } \pazocal{I}^{i})$
\end{enumerate}
We have shown by 2.2.2.3 and 2.2.2.4 that there exists $\textit{EX(pro(a,d), } \pazocal{I}^{i}) \asp{:}$ \\ $\textit{EX(X, } \pazocal{I}^{i})\asp{;}$ in $\textit{CN}$ such that $M_P \models \textit{EX(pro(a,d), } \pazocal{I}^{i}) \asp{:} \textit{EX(X, } \pazocal{I}^{i})\asp{;}$ and therefore that $M_P \models C$.
\item For the case that $\langle A, b \rangle \in \pazocal{A}^{i}(S^{i})$ by \ref{eqCA1} $\asp{holdsat(pow(}b\asp{),} \textit{In}^{i}, j\asp{)}$ - since by the condition of constructing $N$ we have $S^{i}_{j} \models \textit{pow}(b)$ according to \ref{eqDC2}. By construction of $S^{i}_{j}$ we know $M_{P} \models \asp{holdsat(pow(}b\asp{),} \textit{In}^{i}, j\asp{)}$.
\item $\asp{nifluent(}\textit{pro(}b, d\asp{)}, \textit{In}^{i})$ - true by $\textit{pro(}b, d\asp{)} \in \pazocal{F}_{\textit{anorm}}$ and \ref{eqASPMLTrans4}.
\item $\asp{instant(}j\asp{)}$ - According to \ref{eqASPSemTrans16} $\asp{instant(}j\asp{).} \in \Pi^{\textit{base(k)}}$, a fact and therefore $M_{P} \models \asp{instant(}j\asp{)}$.
\end{enumerate}
We have shown that for any $\langle N, n \rangle \in \textit{DC}(S^{i}_{j})$ where $n = \textit{pro}(b, d)$ and $b \in \pazocal{E}$ then we have a ground rule $r = \asp{holdsat(pro(}b, d\asp{)}, \textit{In}^i, j \asp{) :- }$ \\
$\textit{CN}\asp{,} \textit{C} \asp{,} \asp{holdsat(pow(}b\asp{),} \textit{In}^{i}, j\asp{),} \asp{instant(}j\asp{).} \in P^{*}$ and that assuming $S^{i}_{j} \models N$ then $\forall l \in B(r) : M_P \models l$ and thus $M_P \models H(r)$ and by construction $S^{i}_{j} \models n$.
\item \label{proofDCInductiveHyp} \textbf{Inductive hypothesis:} Let $\langle N, n^{\prime} \rangle \in \textit{DC}(S^{i}_{j})$ then $\exists r \in \Pi^{\textit{abstr}}$ s.t. $r = \asp{holdsat(}n^{\prime}, \textit{In}^i, I \asp{) :- }\\
\textit{CN}\asp{,} \textit{C} \asp{,} \asp{holdsat(pow(}b\asp{),} \textit{In}^{i}, I\asp{),} \asp{nifluent(}n^{\prime}, \textit{In}^{i}), \asp{instant(}I\asp{).}$ or $r = \asp{holdsat(}n^{\prime}, \textit{In}^i, I \asp{) :- }\\
\textit{CN}\asp{,} \asp{nifluent(}n^{\prime}, \textit{In}^{i}), \textit{C}\asp{.}$ where $\textit{CN}$ is a set of conditional literals s.t. \\$\forall l \in C : l = \textit{EX(n}, \pazocal{I}^{i}) \asp{:} \textit{EX(X}, \pazocal{I}^{i})\asp{;}, n \in N, X \in \pazocal{X}^{i}$ and $\textit{CN} \neq \emptyset$, and $C$ is an aggregate s.t. $C = \asp{1\{} \textit{CN} \asp{\}}$. The following properties hold:
\begin{enumerate}[label*=\arabic*.]
\item If $\textit{EX(n}, \pazocal{I}^{i}) \asp{:} \textit{EX(X}, \pazocal{I}^{i})\asp{;} \in \textit{CN}$ and $M_P \models \textit{EX(X}, \pazocal{I}^{i})$ then assuming $S^{i}_{j} \models N$ by construction of $S^{i}_{j}$ it is the case that $M_P \models \textit{EX(n}, \pazocal{I}^{i})$. Therefore $M_P \models \textit{CN}$.
\item Assuming $S^{i}_{j} \models N$ then $\exists \textit{EX(n}, \pazocal{I}^{i}) \asp{:} \textit{EX(X}, \pazocal{I}^{i})\asp{;} \in \textit{CN}$ such that $M_P \models  \textit{EX(X}, \pazocal{I}^{i})$ and $M_P \models \textit{EX(n}, \pazocal{I}^{i})$ therefore $M_P \models C = \asp{1\{} \textit{CN} \asp{\}}$.
\item In the case that $\asp{holdsat(pow(}b\asp{),} \textit{In}^{i}, \asp{I)} \in B(r)$ it is the case that $M_P \models \asp{holdsat(pow(}b\asp{),} \textit{In}^{i}, \asp{I)}$.
\item $M_P \models \asp{nifluent(}n^{\prime}, \textit{In}^{i})$
\item It is the case that $M_P \models \asp{instant(}\asp{I)}$.
\end{enumerate}
Thus, assuming $S^{i}_{j} \models N$ then $M_P \models \asp{holdsat(}n^{\prime}, \textit{In}^i, I \asp{)}$ and by construction of $S^{i}_{j}$ it is the case that $n^{\prime} \in S^{i}_{j}$.
\item \textbf{Inductive step 1:} Let $\langle N^{\prime}, n^{\prime} \rangle \in \textit{DC}(S^{i}_{j})$ where $n^{\prime} = \textit{obl}(b, d)$ and $b \in \pazocal{F}^{i}_{\textit{anorm}}$. According to the conditions of \ref{eqDC1} $\exists \langle N, b \rangle \in \textit{DC}(S^{i}_{j})$. By the inductive hypothesis \\$\exists r \in P^{*}$ s.t. $r = \asp{holdsat(}b, \textit{In}^i, I \asp{) :- }$ \\ $\textit{CN}\asp{,} \textit{C} \asp{,} \asp{holdsat(pow(}b\asp{),} \textit{In}^{i}, I\asp{),} \asp{nifluent(}b, \textit{In}^{i}), \asp{instant(}I\asp{).}$ or \\$r = \asp{holdsat(}b, \textit{In}^i, I \asp{) :- }$ \\
$\textit{CN}\asp{,} \textit{C} \asp{,} \asp{nifluent(}b, \textit{In}^{i}), \asp{instant(}I\asp{).}$. Therefore the conditions of \ref{eqASPDCATrans3} are met and we have a rule $r^{\prime} \in \Pi^{\textit{abstr}}$ such that $r^{\prime} = \asp{holdsat(obl(}b, d\asp{)}, \textit{In}^i \asp{,I) :- }\\\textit{CN}^{\prime}, C^{\prime} \asp{,} \asp{holdsat(pow(}b\asp{),} \textit{In}^{i}\asp{, I),} \asp{nifluent(obl(}b, d\asp{)}, \textit{In}^{i}), \asp{instant(I).}$ or $r^{\prime} = \asp{holdsat(obl(}b, d\asp{)}, \textit{In}^i \asp{,I) :- }\\\textit{CN}^{\prime}, C^{\prime} \asp{,} \asp{nifluent(obl(}b, d\asp{)}, \textit{In}^{i}), \asp{instant(I).}$. We will now show that assuming $S^{i}_{j} \models N^{\prime}$ each body literal in $r^{\prime}$ is true.
\begin{enumerate}[label*=\arabic*.]
\item $\textit{CN}^{\prime}$ - According to \ref{eqASPDCATrans3} $\textit{CN}^{\prime} = \{ \textit{EX(obl(a,d), } \pazocal{I}^{i}) \asp{:} c\asp{;} \mid \asp{holdsat(}a, \textit{In}^i \asp{,I) : } c\asp{;} \in \textit{B}(r) \},$ we will show that if $S^{i}_{j} \models c$ then assuming $S^{i}_{j} \models N$ that $S^{i}_{j} \models \textit{EX(obl(a,d), } \pazocal{I}^{i})$.
\begin{enumerate}[label*=\arabic*.]
\item By the inductive hypothesis 2.3. the only conditional literals in $r$ are in $\textit{CN}$ s.t. \\$\asp{holdsat(}a, \textit{In}^i \asp{,I) : } c \asp{;} \in \textit{B}(r)$ iff $\asp{holdsat(}a, \textit{In}^i \asp{,I) : } c \asp{;} \in \textit{CN}$, therefore \\$\textit{CN}^{\prime} = \{ \textit{EX(obl(a,d), } \pazocal{I}^{i}) \asp{:} c \asp{;} \mid \asp{holdsat(}a, \textit{In}^i \asp{,I) : } c\asp{;} \in \textit{CN} \}$. 
\item By the inductive hypothesis 2.3.1. if $\textit{EX(a}, \pazocal{I}^{i}) \asp{:} \textit{EX(X}, \pazocal{I}^{i})\asp{;} \in \textit{CN}$ and $M_P \models \textit{EX(X}, \pazocal{I}^{i})$ then assuming $S^{i}_{j} \models N$ by construction of $S^{i}_{j}$ we have $M_P \models \textit{EX(a}, \pazocal{I}^{i})$. Therefore $\forall \textit{EX(a}, \pazocal{I}^{i}) \asp{:} \textit{EX(X}, \pazocal{I}^{i})\asp{;} \in \textit{CN}$ such that $M_P \models \textit{EX(X}, \pazocal{I}^{i})$ we have $a \in N$. 
\item According to \ref{eqDC2} $N^{\prime}$ is constructed as $N^{\prime} = \{ \textit{obl}(a, d) \mid \; \exists a : a \in N \}$ by 2.4.1.2. and by construction of $\textit{CN}^{\prime}$ in \ref{eqASPDCATrans3} we have for all $\textit{EX(obl(a, d)}, \pazocal{I}^{i}) \asp{:} \textit{EX(X}, \pazocal{I}^{i})\asp{;}$ in $\textit{CN}$ if $M_P \models \textit{EX(X}, \pazocal{I}^{i})$ then $\textit{obl(a, d)} \in N^{\prime}$. 
\item Assuming $N^{\prime} S^{i}_{j} \models N^{\prime}$ then we have $M_P \models \textit{EX(obl(a, d)}, \pazocal{I}^{i}$ and by 2.4.1.3. we have $M_P \models \textit{CN}^{\prime}$.
\end{enumerate}
\item  According to \ref{eqASPDCATrans3} $C^{\prime} = \asp{1\{}\textit{CN}^{\prime}\asp{\}}$, we will show that at least one element of $C^{\prime}$ is modelled by $M_P$ and therefore $C^{\prime}$ is true.
\begin{enumerate}[label*=\arabic*.]
\item By the inductive hypothesis 2.3.1. we have $\exists \textit{EX(a}, \pazocal{I}^{i}) \asp{:} \textit{EX(X}, \pazocal{I}^{i})\asp{;} \in \textit{CN}$ such that $M_P \models  \textit{EX(X}, \pazocal{I}^{i})$. 
\item By 2.4.1. $M_P \models \textit{CN}^{\prime}$ with 2.4.2.1. there exists $\textit{EX(obl(a, d)}, \pazocal{I}^{i})$ \\ $\asp{:} \textit{EX(X}, \pazocal{I}^{i})\asp{;} \in \textit{CN}$ such that $M_P \models\textit{EX(obl(a, d)}, \pazocal{I}^{i})$. 
\item Under the semantics of aggregates one element of $C$ must be true for $C$ to be true, together with 2.4.2.2. we have $M_P \models C = \asp{1\{} \textit{CN} \asp{\}}$.
\end{enumerate}
\item By the inductive hypothesis if $\asp{holdsat(pow(}b\asp{),} \textit{In}^{i}, I\asp{)} \in B(r)$ then $M_P \models \asp{holdsat(pow(}b\asp{),} \textit{In}^{i}, I\asp{)}$.
\item By the inductive hypothesis $M_P \models \asp{nifluent(}\textit{obl(}b, d\asp{)}, \textit{In}^{i})$.
\item By the inductive hypothesis it is the case that $M_P \models \asp{instant(}I\asp{)}$.
\end{enumerate}
Thus, we have shown assuming $S^{i}_{j} \models N^{\prime}$ then $\forall l \in B(r^{\prime}) : M_P \models l$, therefore $M_P \models \asp{holdsat(}n^{\prime}, \textit{In}^i, I \asp{)}$ and by construction of $S^{i}_{j}$ it is the case that $n^{\prime} \in S^{i}_{j}$.
\item \textbf{Inductive step 2:} Let $\langle N^{\prime}, n^{\prime} \rangle \in \textit{DC}(S^{i}_{j})$ where $n^{\prime} = \textit{pro}(b, d)$ and $b \in \pazocal{F}^{i}_{\textit{anorm}}$. According to the conditions of \ref{eqDC2} $N^{\prime}$ is constructed as $\{ \textit{pro}(a, d) \mid \; \exists \langle N, b \rangle, a : \langle N, b \rangle \in \textit{DC}(S^{i}_{j}) \wedge a \in N \}$, $N^{\prime} \neq \emptyset$ and by the inductive hypothesis \\$\forall \langle N, b \rangle \in \textit{DC}(S^{i}_{j}) : \exists r \in P^{*}$ s.t. $r = \asp{holdsat(}b, \textit{In}^i, I \asp{) :- }$ \\ $
\textit{CN}\asp{,} \textit{C} \asp{,} \asp{holdsat(pow(}b\asp{),} \textit{In}^{i}, I\asp{),} \asp{nifluent(}\textit{b} \asp{,} \textit{In}^{i}), \asp{instant(}I\asp{).}$ or \\$r = \asp{holdsat(}b, \textit{In}^i, I \asp{) :- }
\textit{CN}\asp{,} \textit{C} \asp{,} \asp{nifluent(}\textit{b} \textit{In}^{i}), \asp{instant(}I\asp{).}$. Therefore the conditions of \ref{eqASPDCATrans4} are met and we have a rule \\$r^{\prime} \in \Pi^{\textit{abstr}}$ such that $r^{\prime} = \asp{holdsat(pro(}b, d\asp{)}, \textit{In}^i \asp{,I) :- }\\\textit{CN}^{\prime}, C^{\prime} \asp{,} \asp{holdsat(pow(}b\asp{),} \textit{In}^{i}\asp{, I),} \asp{nifluent(}\textit{pro(}b, d\asp{)}, \textit{In}^{i}), \asp{instant(I).}$ or a rule \\$r^{\prime} \in \Pi^{\textit{abstr}}$ such that $r^{\prime} = \asp{holdsat(pro(}b, d\asp{)}, \textit{In}^i \asp{,I) :- }\\\textit{CN}^{\prime}, C^{\prime} \asp{,} \asp{nifluent(}\textit{pro(}b, d\asp{)}, \textit{In}^{i}), \asp{instant(I).}$. We will now show that assuming $S^{i}_{j} \models N^{\prime}$ each body literal in $r^{\prime}$ is true.
\begin{enumerate}[label*=\arabic*.]
\item $\textit{CN}^{\prime}$ - According to \ref{eqASPDCATrans4} $\textit{CN}^{\prime} = \{ \textit{EX(pro(a,d), } \pazocal{I}^{i}) \asp{:} c\asp{;} \mid r \in R,
\asp{holdsat(}a, \textit{In}^i \asp{,I) : }$ \\ $c\asp{;} \in B(r) \}$ where $R = \{ r \in \Pi^{\textit{abstr}} : \textit{H}(r) = \asp{holdsat(}b\asp{,} \textit{In}^{i}, \asp{I)} \}$. We will show that if $S^{i}_{j} \models c$ then assuming $S^{i}_{j} \models N^{\prime}$ that $S^{i}_{j} \models \textit{EX(pro(a,d), } \pazocal{I}^{i})$.
\begin{enumerate}[label*=\arabic*.]
\item By the inductive hypothesis, and since according to Definition~\ref{defASPDCATrans} there are no other rules in $\Pi_{\textit{abstr}}$ not covered by the base cases 1 and 2 and the inductive hypothesis we have the following bi-directional property $\langle N, b \rangle \in \textit{DC}(S^{i}_{j})$ iff $\exists r \in P^{\textit{abstr}}$ s.t. \\$r = \asp{holdsat(}b, \textit{In}^i, I \asp{) :- }
\textit{CN}\asp{,} \textit{C} \asp{,} \asp{holdsat(pow(}b\asp{),} \textit{In}^{i}, I\asp{),} \asp{instant(}I\asp{).}$.
\item By the inductive hypothesis 2.3.1. for all \\$r \in P^{\textit{abstr}}$ s.t. $H(r) = \asp{holdsat(}b, \textit{In}^i, I \asp{)}$ if $\textit{EX(a}, \pazocal{I}^{i}) \asp{:} \textit{EX(X}, \pazocal{I}^{i})\asp{;} \in \textit{CN}$ and $M_P \models \textit{EX(X}, \pazocal{I}^{i})$ then $a \in N$
\item According to \ref{eqDC2} $N^{\prime}$ is constructed as $N^{\prime} = \{ \textit{pro}(a, d) \mid \exists \langle N, b \rangle, a : \langle N, b \rangle \in \textit{DC}(S^{i}_{j}) \wedge a \in N \}$ and by 2.5.1.2. we have for all \\$\textit{EX(pro(a, d)}, \pazocal{I}^{i}) \asp{:} \textit{EX(X}, \pazocal{I}^{i})\asp{;}$ in $\textit{CN}^{\prime}$ if $S^{i}_{j} \models X$ then by construction of $S^{i}_{j}$ we have $M_P \models \textit{EX(X}, \pazocal{I}^{i})$, assuming $N^{\prime} \subseteq S^{i}_{j}$ we have $M_P \models \textit{EX(pro}(b, d), \pazocal{I}^{i})$. Therefore, $M_P \models \textit{CN}^{\prime}$.
\end{enumerate}
\item According to \ref{eqASPDCATrans4} $C^{\prime} = \asp{1\{}\textit{CN}^{\prime}\asp{\}}$ we will show that at least one element of $C^{\prime}$ is modelled by $M_P$ and therefore $C^{\prime}$ is true.
\begin{enumerate}[label*=\arabic*.]
\item By the inductive hypothesis 2.3.2. we have $\exists \textit{EX(a}, \pazocal{I}^{i}) \asp{:} \textit{EX(X}, \pazocal{I}^{i})\asp{;} \in \textit{CN}^{\prime}$ such that $M_P \models  \textit{EX(X}, \pazocal{I}^{i})$. 
\item By 2.5.1. $M_P \models \textit{CN}^{\prime}$ and $\textit{EX(pro(a, d)}, \pazocal{I}^{i}) \asp{:} \textit{EX(X}, \pazocal{I}^{i})\asp{;} \in \textit{CN}$ and by 2.5.2.1 we have $M_P \models\textit{EX(X}, \pazocal{I}^{i})$ therefore under the semantics of aggregates we have $M_P \models C = \asp{1\{} \textit{CN} \asp{\}}$.
\end{enumerate}
\item By the inductive hypothesis it is the case that $M_P \models \asp{holdsat(pow(}b\asp{),} \textit{In}^{i}, I\asp{)}$.
\item By the inductive hypothesis $M_P \models \asp{nifluent(}\textit{pro(}b, d\asp{)}, \textit{In}^{i})$.
\item By the inductive hypothesis it is the case that $M_P \models \asp{instant(}I\asp{)}$.
\end{enumerate}
Thus, we have shown assuming $S^{i}_{j} \models N^{\prime}$ then $\forall l \in B(r^{\prime}) : M_P \models l$, therefore $M_P \models \asp{holdsat(}n^{\prime}, \textit{In}^i, I \asp{)}$ and by construction of $S^{i}_{j}$ it is the case that $n^{\prime} \in S^{i}_{j}$.
\end{enumerate}
Therefore we have shown that if $\langle N, n \rangle \in \textit{DC}(S^{i}_{j})$ and $S^{i}_{j} \models N$ then $n \in \overline{\textit{DC}}^{i}(S^{i}_{j})$, consequently $n \in S^{i}_{j}$ and thus $\overline{\textit{DC}}^{i}(S^{i}_{j}) \subseteq S^{i}_{j}$.
\end{enumerate}
We have proven that $S^{i}_{j} = \overline{\textit{DC}}^{i}(S^{i}_{j})$.
\end{proof}

\subsection{Soundness Proof}
\label{proofSound}

\begin{proof}{\textbf{Theorem~\ref{theorSound} Soundness}} We need to show
\begin{enumerate}
\item According to \ref{eqIS1} $\forall i \in [1, n] : S^{i}_0 \subseteq \Delta^{i}$, $\exists \langle h, i \rangle \in R, n \in (\pazocal{F}^{h}_{\textit{cnorm}} \cup \pazocal{F}^{h}_{\textit{anorm}}) \cap \pazocal{F}^{i}_{\textit{ninert}} : n \in S^{h}_{0} \Rightarrow n \in S^{i}_{0}$, $\forall i \in [1,n] : S^{i}_0 = \textit{FD}^{i}(S^{i}_0)$ and $\forall i \in [1,n] : S^{i}_0 = \overline{\textit{DC}}^{i}(S^{i}_0)$.
\item According to Definition~\ref{defMLGModel} $\forall i \in [1, n], \forall j \in [1,k] : E^{i}_j = \textit{GR}^{i}(S^{i}_{j-1}, \{ \textit{se}^{i}_{j} \})$. Where $\textit{GR}^{i}$ is the event generation operation for an institution $\pazocal{I}^{i}$  w.r.t. $E = \langle E^{1}_{j}, ..., E^{n}_{j}\rangle$.
\item According to Definition~\ref{defMLGModel} $\forall i \in [1, n], \forall j \in [1,k+1] : S^{i}_j = \textit{TR}^{i}(S^{i}_{j-1}, E^{i}_{j})$. Where $\textit{TR}^{i}$ is the state transition operation for an institution $\pazocal{I}^{i}$  w.r.t. $S = \langle S^{1}_{j}, ..., S^{n}_{j}\rangle$.
\end{enumerate}
Each condition is dealt with separately:
\begin{enumerate}
\item $\forall i \in [1, n] : S^{i}_0 \subseteq \Delta^{i}$, $\exists \langle h, i \rangle \in R, n \in (\pazocal{F}^{h}_{\textit{cnorm}} \cup \pazocal{F}^{h}_{\textit{anorm}}) \cap \pazocal{F}^{i}_{\textit{ninert}} : n \in S^{h}_{0} \Rightarrow n \in S^{i}_{0}$, $\forall i \in [1,n] : S^{i}_0 = \textit{FD}^{i}(S^{i}_0)$ and $\forall i \in [1,n] : S^{i}_0 = \overline{\textit{DC}}^{i}(S^{i}_0)$:
\begin{enumerate}[label*=\arabic*.]
\item $\Delta^{i} \subseteq S^{i}_{0}$ - if $f \in \Delta^{i}$ then by \ref{eqASPMLTrans10} there is a rule with $r \in \Pi^{\pazocal{ML}(k)}$ such that $\asp{holdsat(}f, \textit{In}^{i}, I) \in H(r)$ and only one literal $\asp{start(I)} \in B(r)$ in the body, by \ref{eqASPSemTrans16} $\asp{start}(0) \in \Pi^{\pazocal{ML}(k)}$ is a fact and therefore $M_P \models \asp{holdsat(}f, \textit{In}^{i}, 0) $ and by construction of $S^{i}_{j}$ we have $f \in S^{i}_{0}$.
\item $\exists \langle h, i \rangle \in R, n \in (\pazocal{F}^{h}_{\textit{cnorm}} \cup \pazocal{F}^{h}_{\textit{anorm}}) \cap \pazocal{F}^{i}_{\textit{ninert}} : n \in S^{h}_{0} \Rightarrow n \in S^{i}_{0}$:
\begin{enumerate}[label*=\arabic*.]
\item According to \ref{eqASPMLTrans13} we have an AnsProlog rule \\$r = \asp{holdsat(} n \asp{, }\textit{In}^i \asp{, I) :- } \asp{holdsat(} n\asp{, }\textit{In}^h\asp{, I).}$
\item By 1.2.1. and construction of $S^{h}_{0}$ we have $M_P \models \asp{holdsat(} n\asp{, }\textit{In}^h\asp{, I)}$.
\item By \ref{eqASPSemTrans16} we have $\asp{instant(0)}. \in \Pi^{\pazocal{ML}(k)}$, a fact and therefore $M_P \models \asp{instant(0)}$ and thus $r$ is grounded s.t. $r = \asp{holdsat(} n \asp{, }\textit{In}^i \asp{, 0) :- }$ \\ $\asp{holdsat(} n\asp{, }\textit{In}^h\asp{, 0).} \in \Pi^{*}$.
\item By 1.2.2. and 1.2.3. $\forall l \in B(r^{\prime}) : M_P \models l$, therefore $M_P \models H(r^{\prime})$ and by construction of $S^{i}_{0}$ we have $f \in S^{i}_{0}$.
\end{enumerate}
We have shown $\exists \langle h, i \rangle \in R, n \in (\pazocal{F}^{h}_{\textit{cnorm}} \cup \pazocal{F}^{h}_{\textit{anorm}}) \cap \pazocal{F}^{i}_{\textit{ninert}} : n \in S^{h}_{0} \Rightarrow n \in S^{i}_{0}$.
\item $\forall i \in [1,n] : S^{i}_0 = \textit{FD}^{i}(S^{i}_0)$:
\begin{enumerate}
\item By \ref{eqDepFl1} and construction $S^{i}_0 \subseteq \textit{FD}^{i}(S^{i}_0)$.
\item By \ref{eqDepFl2} if $\exists X \in \pazocal{X}, f \in S^{i}_0, f^{\prime} \in \pazocal{D}^{i}(X, f) : S^{i}_0 \models X$ then $f^{\prime} \in S^{i}_0$.
\item By 1.3.ii and \ref{eqASPMLTrans12} we have an AnsProlog rule $r = \asp{holdsat(} f^{\prime}\asp{, }\textit{In}^i \asp{, I) :- } \\
\asp{holdsat(} f\asp{, }\textit{In}^i\asp{, I),} \; \textit{EX(X,} \pazocal{I}^i), \asp{instant(I).}$.
\item By  \ref{eqASPSemTrans16} we have $\asp{instant(0)}. \in \Pi^{\pazocal{ML}(k)}$, a fact and therefore $M_P \models \asp{instant(0)}$ and thus $r$ is grounded s.t. $r = \asp{holdsat(} f^{\prime}\asp{, }\textit{In}^i \asp{, 0) :- }$ \\ $\asp{holdsat(} f\asp{, }\textit{In}^i\asp{, 0),} \; \textit{EX(X,} \pazocal{I}^i), \asp{instant(0).} \in \Pi^{*}$.
\item By 1.3.iii and construction of $S^{i}_0$ we have $M_P \models \textit{EX(X,} \pazocal{I}^i)$ and $M_P \models \asp{holdsat(} f\asp{, }\textit{In}^i\asp{, I),}$.
\item By 1.3.iii, 1.3.iv and 1.3.v we have $\forall l \in B(r) : M_P \models l$, therefore $M_P \models H(r)$ and by construction of $S^{i}_{0}$ we have $f^{\prime} \in S^{i}_{0}$.
\end{enumerate}
By 1.3.i awe have $S^{i}_0 \subseteq \textit{FD}^{i}(S^{i}_0)$ and by 1.3.ii and 1.3.vi we have $ \textit{FD}^{i}(S^{i}_0) \subseteq S^{i}_0$, therefore we have shown $S^{i}_0 = \textit{FD}^{i}(S^{i}_0)$.
\item By Lemma~\ref{theoremAbstraction} we have $S^{i}_{0} = \overline{\textit{DC}}^{i}(S^{i}_{0})$.
\end{enumerate}
By 1.1. and 1.2. and 1.3. we have proven $\forall i \in [1, n] : S^{i}_0 \subseteq \Delta^{i}$, $\exists \langle h, i \rangle \in R, n \in (\pazocal{F}^{h}_{\textit{cnorm}} \cup \pazocal{F}^{h}_{\textit{anorm}}) \cap \pazocal{F}^{i}_{\textit{ninert}} : n \in S^{h}_{0} \Rightarrow n \in S^{i}_{0}$, $\forall i \in [1,n] : S^{i}_0 = \textit{FD}^{i}(S^{i}_0)$ and $\forall i \in [1,n] : S^{i}_0 = \overline{\textit{DC}}^{i}(S^{i}_0)$.
\item $\forall i \in [1, n], \forall j \in [k] : E^{i}_{j} = \textit{GR}^{i}(S^{i}_{j}, \{ \textit{se}^{i}_{j} \})$ - we prove by showing that $\textit{GR}^{i}(S^{i}_{j}, \{ \textit{se}^{i}_{j} \}) \subseteq E^{i}_{j}$ and $E^{i}_{j} \subseteq \textit{GR}^{i}(S^{i}_{j}, \{ \textit{se}^{i}_{j} \})$ separately.
\begin{enumerate}[label*=\arabic*.]
\item $\textit{GR}^{i}(S^{i}_{j}, \{ \textit{se}^{i}_{j} \}) \subseteq E^{i}_{j}$ - we will show that in Definition~\ref{defGR} all events \\ $e^{\prime} \in \textit{GR}^{i}(S^{i}_{j}, \{ \textit{se}^{i}_{j} \})$ according to \ref{eqGR10}-\ref{eqGR18} are in $E^{i}_{j}$ due to an applied rule $r \in \Pi^{\pazocal{ML}(k)}$ with $\asp{occurred(}e^{\prime}, \textit{In}^{i}, I\asp{)} \in H(r)$ and by construction of $E^{i}_{j}$.
\newcounter{grNeccProofCounter}
\begin{enumerate}[label*=\arabic*.]
\item According to \ref{eqGR10} $e^{\prime} = \textit{now}$ is necessarily in $\textit{GR}^{i}(S^{i}_{j}, \{ \textit{se}^{i}_{j} \})$. According \ref{eqASPMLTrans3} we have an AnsProlog rule $r \in \Pi^{\textit{base}(k)}$ and thus $r \in \Pi^{\pazocal{ML}(k)}$ s.t. $H(r) = \asp{occurred(}\textit{now}, \asp{In}, \asp{I)}$ and $B(r) = \{ \asp{instant(I)}, \asp{inst(In)}\}$. According to \ref{eqASPSemTrans16} we have facts $\asp{instant(j)} \in P^{*}$ and \ref{eqASPMLTrans1} $\asp{inst}(\textit{In}^{i}) \in P^{*}$. Thus we have $M_P \models \asp{occurred(}\textit{now}, \textit{In}^{i}, j\asp{)}$ and by construction of $E^{i}_{j}$, $\textit{now} \in E^{i}_{j}$.
\item According to \ref{eqGR11} $e^{\prime} \in \{ \textit{se}^{i}_{j} \}$ is necessarily in $\textit{GR}^{i}(S^{i}_{j}, \{ \textit{se}^{i}_{j} \})$, we will show $\textit{se}^{i}_{j} \in E^{i}_{j}$.
\begin{enumerate}[label*=\arabic*.]
\item By \ref{eqASPSemTrans10} we have a rule $r \in \Pi^{\pazocal{ML}(k)}$ such that \\$H(r) = \asp{observed(E, In, I)}$, by \ref{eqASPCompTraceTrans} we have a fact $\asp{observed(}e, j\asp{).} \in \Pi^{\pazocal{ML}(k)}$, by \ref{eqASPMLTrans1} $\asp{inst}(\textit{In}^{i}) \in \Pi^{\pazocal{ML}(k)}$ and therefore we have $M_P \models \asp{observed(}e, \textit{In}^{i}, j\asp{)}$.
\item According to Definition~\ref{defSynchTrace} either $\textit{se}^{i}_{j} \in \pazocal{E}^{i}_{\textit{obs}}$ or $\textit{se}^{i}_{j} = e_{\textit{null}}$.
\item If $\textit{se}^{i}_{j} \in \pazocal{E}^{i}_{\textit{obs}}$ then by \ref{eqASPMLTrans2} we have a fact $\asp{evtype(}e\asp{,} \textit{In}^{i}\asp{ex).} \in \Pi^{\pazocal{ML}(k)}$. By \ref{eqASPSemTrans4} we have a rule $r \in \Pi^{\pazocal{ML}(k)}$ such that $H(r) = \asp{occurred(E, In, I)}$ and the aforementioned literals modelled by $M_P$ we have \\$M_P \models \asp{occurred(}e, \textit{In}^{i}, j \asp{)}$ where $e \in \pazocal{E}^{i}$. 
\item If $\textit{se}^{i}_{j} = e_{\textit{null}}$ then by Definition~\ref{defSynchTrace} we know $e \not \in \pazocal{E}^{i}$, thus according to the translation in Definition~\ref{defASPMLTrans} we have $\asp{evtype(}e, \textit{In}^{i}, \asp{ex).} \not \in \Pi^{\pazocal{ML}(k)}$ and $\forall r \in \Pi^{*} : \asp{evtype(}e, \textit{In}^{i}, \asp{ex)} \neq H(r)$. Therefore $M_P \not \models \asp{evtype(}e, \textit{In}^{i}, \asp{ex)}$. Thus, we have by $\ref{eqASPSemTrans5}$ a rule $r \in \Pi^{\pazocal{ML}(k)}$ such that $H(r) = \asp{occurred(null, In, I)}$ where $\forall l \in B(r) : M_P \models l$ and the head is ground s.t. $M_P \models \asp{occurred(null,} \textit{In}^{i}, j\asp{)}$. 
\item By 3.1.2.3 and 3.1.2.4. and construction of $E^{i}_{j}$ we have $\textit{se}^{i}_{j} \in E^{i}_{j}$.
\end{enumerate}
\setcounter{grNeccProofCounter}{\theenumi}
\end{enumerate}
Conditions \ref{eqGR13}-\ref{eqGR17} depend recursively on an event already being in \\ $\textit{GR}^{i}(S^{i}_{j}, \{ \textit{se}^{i}_{j} \})$ according to \ref{eqGR10} - \ref{eqGR18} or non-recursively depending on $S^{i}_{j} \models l$  for some literal $l$ in the case of \ref{eqGR14}-\ref{eqGR17}. We have already given the base cases for if according to \ref{eqGR10} - \ref{eqGR11} $e^{\prime} \in \textit{GR}^{i}(S^{i}_{j}, \{ \textit{se}^{i}_{j} \})$ then $e^{\prime} \in E^{i}_{j}$. We make the inductive hypothesis that $\forall i \in [1,n]$ if according to \ref{eqGR10}-\ref{eqGR18} $e^{\prime} \in \textit{GR}^{i}(S^{i}_{j}, \{ \textit{se}^{i}_{j} \})$ then $e^{\prime} \in E^{i}_{j}$. The inductive steps are given for \ref{eqGR13}-\ref{eqGR18} as follows:
\begin{enumerate}[label*=\arabic*.]
\setcounter{enumiii}{\thegrNeccProofCounter - 1}
\item \ref{eqGR13} -
\begin{enumerate}[label*=\arabic*.]
\item According to \ref{eqGR13} we have $e^{\prime} \in \textit{GR}^{i}(S^{i}_{j}, \{ \textit{se}^{i}_{j} \})$ if \\$X \in \pazocal{X}^{i} \wedge$ \\ $e \in \textit{GR}^{i}(S^{i}_{j}, \{ \textit{se}^{i}_{j} \} \wedge S^{i}_{j} \models X \wedge e^{\prime} \in \pazocal{G}(X, e) \wedge S \models \textit{pow}(e^{\prime})$. 
\item By 2.1.3.1. and \ref{eqASPMLTrans9} we have a rule $r \in \Pi^{\pazocal{ML}(k)}$ such that $H(r) = \asp{occurred}(e^{\prime}, \textit{In}^{i}, \asp{I)}$. 
\item By 2.1.3.1. we have $S^{i}_{j} \models X$ and $S^{i}_{j} \models \textit{pow}(e^{\prime})$, and by the construction of $S^{i}_{j}$ we have $M_P \models \textit{EX(X,}\pazocal{I}^{i}\textit{)}$ and $M_P \models \asp{holdsat(pow(}e^{\prime}), \textit{In}^{i}, \asp{I)}$. 
\item By \ref{eqASPSemTrans16} we know we have a fact in $\Pi^{\pazocal{ML}(k)}$ such that \\$M_P \models \asp{instant(j)}$. 
\item By the inductive hypothesis we assume if $e \in \textit{GR}^{i}(S^{i}_{j}, \{ \textit{se}^{i}_{j} \})$ then $e \in E^{i}_{j}$, thus by construction of $E^{i}_{j}$ we have $M_P \models \asp{occurred}(e, \textit{In}^{i}, j\asp{)}$. 
\item By 2.1.3.2., 2.1.3.3., 2.1.3.4. and 2.1.3.5. all body literals of $r$ are true and therefore \\$M_P \models \asp{occurred}(e^{\prime}, \textit{In}^{i}, j\asp{)}$ and by construction of $E^{i}_{j}$ we have $e^{\prime} \in E^{i}_{j}$.
\end{enumerate}
\item \ref{eqGR14}-\ref{eqGR17} are dealt together due to their similarity 
\begin{enumerate}[label*=\arabic*.]
\item According to \ref{eqGR14}-\ref{eqGR17} $e^{\prime} \in \textit{GR}^{i}(S^{i}_{j}, \{ \textit{se}^{i}_{j} \})$ if $S^{i}_{j} \models f$ where $f = \textit{obl(a, d)}$ (\ref{eqGR14}, \ref{eqGR15}) or $f = \textit{pro(a, d)}$ (\ref{eqGR16}, \ref{eqGR17}), $e = \textit{disch(f)}$ (\ref{eqGR14}, \ref{eqGR16}) or $e = \textit{viol(f)}$ (\ref{eqGR15}, \ref{eqGR17}). 
\item The other conditions either depend on $e^{\prime} \in \textit{GR}^{i}(S^{i}_{j}, \{ \textit{se}^{i}_{j} \})$ for which by the inductive hypothesis we assume $e \in E^{i}_{j}$ and by construction of $E^{i}_{j}$, $M_P \models \asp{occurred}(e, \textit{In}^{i}, j\asp{)}$ 
\item Or, depend on some $f^{\prime} \in S^{i}_{j}$ for which we have by construction of  $S^{i}_{j}$, $M_P \models \asp{holdsat}(f^{\prime}, \textit{In}^{i}, j\asp{)}$. 
\item In the case of \ref{eqGR15} and \ref{eqGR17} the conditions also depend on $\textit{disch}(f) \not \in \textit{GR}^{i}(S^{i}_{j}, \{ \textit{se}^{i}_{j} \})$, assuming that $E^{i}_{j} \subseteq \textit{GR}^{i}(S^{i}_{j}, \{ \textit{se}^{i}_{j} \})$ (subsequently proven) then if the conditions of \ref{eqGR15} or \ref{eqGR17} are met we have $\textit{disch}(f) \not \in E^{i}_{j}$ and by construction of $E^{i}_{j}$, $M_P \not \models \asp{occurred}(\asp{disch(}f\asp{),} \textit{In}^{i}, j\asp{)}$. 
\item According to \ref{eqASPSemTrans11} - \ref{eqASPSemTrans14} there is an AnsProlog rule $r \in \Pi^{\pazocal{ML}(k)}$ such that $H(r) = \asp{occurred}(e^{\prime}\asp{,} \textit{In}^{i}, j\asp{)}$.
\item By 2.1.3.1. to 2.1.3.5. all body literals of $r$ are true as and therefore $M_P \models \asp{occurred}(e^{\prime}\asp{,} \textit{In}^{i}, j\asp{)}$ and by construction of $E^{i}_{j}$ we have $e^{\prime} \in E^{i}_{j}$.
\end{enumerate}
\item \ref{eqGR18} -
\begin{enumerate}[label*=\arabic*.]
\item By \ref{eqASPMLTrans14} it is necessarily the case that  $e^{\prime} \in \textit{GR}^{i}(S^{i}_{j}, \{ \textit{se}^{i}_{j} \})$ if $\exists \langle h, i \rangle \in R, e^{\prime} \in \pazocal{E}^{h}_{\textit{norm}} \cap \pazocal{E}^{i}_{\textit{norm}}$.
\item By 2.1.4.1. and \ref{eqASPMLTrans14} we have all the conditions for an AnsProlog rule $r \in \Pi^{*}$ such that \\$H(r) = \asp{occurred}(e^{\prime}\asp{,} \textit{In}^{i}, j\asp{)}$ and $B(r) = \{ \asp{occurred(} e\asp{, }\textit{In}^h\asp{, I).} \}$. 
\item By the inductive hypothesis we assume for $h \in [1,n]$ that if \\$e \in \textit{GR}^{h}(S^{h}_{j}, \{ \textit{se}^{h}_{j} \})$ then $e \in E^{h}_{j}$. Hence, by 2.1.4.1. and construction of $E^{h}_{j}$ we have $M_P \models \asp{occurred(}e, \textit{In}^{h}, j \asp{)}$.ff
\item By 2.1.4.3. all body literals of $r$ are true and we have \\$M_P \models \asp{occurred}(e^{\prime}\asp{,} \textit{In}^{i}, j\asp{)}$.
\end{enumerate}
\end{enumerate}
We have proven $\textit{GR}^{i}(S^{i}_{j}, \{ \textit{se}^{i}_{j} \}) \subseteq E^{i}_{j}$.
\item $E^{i}_{j} \subseteq \textit{GR}^{i}(S^{i}_{j}, \{ \textit{se}^{i}_{j} \})$ - we will prove that if $e^{\prime} \in E^{i}_{j}$ then $e^{\prime}$ is one of the events described by the minimality constraints on $\textit{GR}^{i}$, \ref{eqGR1}-\ref{eqGR9}, and thus \\ $e^{\prime} \in \textit{GR}^{i}(S^{i}_{j}, \{ \textit{se}^{i}_{j} \})$. We prove by showing that for each applied rule with $\asp{occurred(}e^{\prime}\asp{,}\textit{In}^{i}\asp{,} j\asp{)}$ in the head causes $e^{\prime} \in E^{i}_{j}$ such that $e^{\prime}$ is one of the literals in \ref{eqGR1}-\ref{eqGR9}. The relevant rules are \ref{eqASPSemTrans3}-\ref{eqASPSemTrans5} and \ref{eqASPSemTrans11}-\ref{eqASPSemTrans16}. For each of the rules being applied causing $e^{\prime} \in E^{i}_{j}$ we show $e^{\prime} \in \textit{GR}^{i}(S^{i}_{j}, \{ \textit{se}^{i}_{j} \})$:
\begin{enumerate}[label*=\arabic*.]
\item \ref{eqASPSemTrans3} - by the construction of $E^{i}_{j}$, $e^{\prime} = \textit{now}$. According to \ref{eqGR1} $\textit{now} \in \textit{GR}^{i}(S^{i}_{j}, \{ \textit{se}^{i}_{j} \})$.
\item \ref{eqASPSemTrans4} - 
\begin{enumerate}[label*=\arabic*.]
\item By \ref{eqASPSemTrans4} the body literals $M_P \models \asp{evtype(}e^{\prime}\asp{,} \textit{In}^{i} \asp{,ex} \asp{)}$ and \\ $M_P \models \asp{observed(}e^{\prime}\asp{,} \textit{In}^{i} \asp{,} j \asp{)}$, must be in the head of an applied rule in $\Pi^{\pazocal{ML}(k)}$. 
\item If $M_P \models \asp{evtype(}e^{\prime}\asp{,} \textit{In}^{i} \asp{,ex} \asp{)}$ then there must be a fact produced by \ref{eqASPMLTrans2} implying $e^{\prime} \in \pazocal{E}_{\textit{obs}}$. 
\item If $M_P \models \asp{observed(}e^{\prime}\asp{,} \textit{In}^{i} \asp{,} j \asp{)}$ then rule \ref{eqASPSemTrans10} is applied implying $M_P \models \asp{observed(}e^{\prime}\asp{,} j \asp{)}$.
\item By Definition~\ref{defASPCompTraceTrans} we have for the composite trace $\textit{ctr} = \langle e_0, ..., e_k \rangle$ a fact $\asp{observed(}e_j\asp{,} j \asp{).} \in \Pi^{\pazocal{ML}(k)}$. 
\item By 2.2.2.4. and \ref{defASPCompTraceTrans} $e^{\prime} = e_j$ or the rule \ref{eqASPSemTrans6} is applied such that $M_P \models \asp{observed(}e\asp{,} j \asp{)}$ where $e \neq e_j$ which would violate the constraint \ref{eqASPSemTrans7} and thus $M_P$ would not be an answer-set. 
\item By 2.2.2.5. and \ref{defASPCompTraceTrans} $\asp{observed(}e_j\asp{,} j \asp{).} \in \Pi^{\pazocal{ML}(k)}$,  $e^{\prime} = e_j$ and by 2.2.2.1. $M_P \models \asp{evtype(}e^{\prime}\asp{,} \textit{In}^{i} \asp{,ex} \asp{).} \in P$ and therefore by \ref{eqASPMLTrans2} $e_j \in \pazocal{E}^{i}$. 
\item Since $e_j \in \pazocal{E}^{i}$ we have by Definition~\ref{defSynchTrace} and 2.2.2.3. that $e^{\prime} = e_j = \textit{se}^{i}_{j}$.
\item According to \ref{eqGR2} $\textit{se}^{i}_{j} \in \textit{GR}^{i}(S^{i}_{j}, \{ \textit{se}^{i}_{j} \})$.
\end{enumerate}
\item \ref{eqASPSemTrans5} - 
\begin{enumerate}[label*=\arabic*.]
\item By \ref{eqASPSemTrans5} and construction of $E^{i}_{j}$ we have $e^{\prime} = e_{\textit{null}}$, \\$M_P \not \models \asp{evtype(}e\asp{,} \textit{In}^{i} \asp{,ex} \asp{)}$ and $M_P \models \asp{observed(}e\asp{,} \textit{In}^{i} \asp{,} j \asp{)}$.
\item By 2.2.3.1. $M_P \not \models \asp{evtype(}e\asp{,} \textit{In}^{i} \asp{,ex} \asp{)}$ so \ref{eqASPMLTrans2} has not produced a fact implying $e \not \in \pazocal{E}_{\textit{obs}}$. 
\item By 2.2.3.1. $M_P \models \asp{observed(}e\asp{,} \textit{In}^{i} \asp{,} j \asp{)}$ then rule \ref{eqASPSemTrans10} is applied implying $M_P \models \asp{observed(}e\asp{,} j \asp{)}$. 
\item By Definition~\ref{defASPCompTraceTrans} we have for the composite trace $\textit{ctr} = \langle e_0, ..., e_k \rangle$ a fact $\asp{observed(}e_j\asp{,} j \asp{).} \in \Pi^{\pazocal{ML}(k)}$. Therefore, we either have by \ref{defASPCompTraceTrans} that $e = e_j$ or the rule \ref{eqASPSemTrans6} is applied such that $M_P \models \asp{observed(}e\asp{,} j \asp{)}$ where $e \neq e_j$ which would violate the constraint \ref{eqASPSemTrans7} and thus $M_P$ would not be an answer-set. Therefore $e = e_j$.
\item By \ref{defASPCompTraceTrans} we have that $\asp{observed(}e_j\asp{,} j \asp{).} \in \Pi^{\pazocal{ML}(k)}$, and $e = e_j$ and thus \\$M_P \not \models \asp{evtype(}e_j\asp{,} \textit{In}^{i} \asp{,ex} \asp{)}$. This implies by \ref{eqASPMLTrans2} that $e = e_j \not \in \pazocal{E}^{i}_{\textit{obs}}$, therefore according to Definition~\ref{defSynchTrace} given the synchronised trace $\textit{str} = \langle \textit{se}_0, ..., \textit{se}_k \rangle$ for $\pazocal{I}^{i}$ of $\textit{ctr}$ we have $\textit{se}_{j} = e_{\textit{null}}$. 
\item Since $e^{\prime} = e_{\textit{null}} = \textit{se}_{j}$ then according to \ref{eqGR2} $e^{\prime} \in \textit{GR}^{i}(S^{i}_{j}, \{ \textit{se}^{i}_{j} \})$.
\end{enumerate}
\item \ref{eqASPSemTrans11}-\ref{eqASPSemTrans14} - 
\begin{enumerate}[label*=\arabic*.]
\item By \ref{eqASPSemTrans11}-\ref{eqASPSemTrans14} and construction of $E^{i}_{j}$ we have $e^{\prime} = \textit{disch(f)}$ or $e^{\prime} = \textit{viol(f)}$ for some $f = \textit{obl(a, d)}$ or $f = \textit{pro(a, d)}$. 
\item According to \ref{eqASPSemTrans11}-\ref{eqASPSemTrans14} we have $M_P \models \asp{holdsat(}f\asp{,In,I)}$ and by construction of $S^{i}_{j}$, $S^{i}_{j} \models f$. 
\item Two rules, \ref{eqASPSemTrans12} and \ref{eqASPSemTrans14}, if applied depend on \\$M_P \not \models \asp{occurred(disch(}f\asp{)},In^{i},j\asp{)}$, by construction of $E^{i}_{j}$ we therefore have $\textit{disch(f)} \not \in E^{i}_{j}$.
\item By 3.1. $\textit{GR}^{i}(S^{i}_{j}, \{ \textit{se}^{i}_{j} \}) \subseteq E^{i}_{j}$ therefore if $e \in \textit{GR}^{i}(S^{i}_{j}, \{ \textit{se}^{i}_{j} \})$ then $e \in E^{i}_{j}$ and by contraposition if $\textit{disch(f)} \not \in E^{i}_{j}$ then $\textit{disch(f)} \not \in \textit{GR}^{i}(S^{i}_{j}, \{ \textit{se}^{i}_{j} \})$. 
\item If one of \ref{eqASPSemTrans11}-\ref{eqASPSemTrans14} is applied then we either have \\$M_P \models \asp{holdsat(}p\asp{,In,I)}$ \\ or $M_P \models \asp{occurred(}p\asp{,}\textit{In}^{i}\asp{,}j\asp{)}$ where $p = a$ for \ref{eqASPSemTrans11} and \ref{eqASPSemTrans14} and $p = d$ for \ref{eqASPSemTrans12} and \ref{eqASPSemTrans13}. 
\item If we have $M_P \models \asp{holdsat(}p\asp{,In,I)}$ then the applied rule is a base case and by construction of $S^{i}_{j}$ we have $S^{i}_{j} \models p$.
\item If we have $M_P \models \asp{occurred(}p\asp{,In,I)}$ then the applied rule depends recursively on another applied rule, the base cases are \ref{eqASPSemTrans3}-\ref{eqASPSemTrans5} and \ref{eqASPSemTrans11}-\ref{eqASPSemTrans14} (which we prove separately).
\item If there is an applied rule $r \in \Pi^{\pazocal{ML}(k)}$ such that \\$H(r) = \asp{occurred(}e\asp{,}\textit{In}^{i}\asp{,}j\asp{)}$ for some $e$ then by construction of $E^{i}_{j}$ we have $e \in E^{i}_{j}$ we make the inductive hypothesis that $e \in  \textit{GR}^{i}(S^{i}_{j}, \{ \textit{se}^{i}_{j} \})$.
\item We give the inductive step for a rule $r$ \ref{eqASPSemTrans11} -\ref{eqASPSemTrans14} (other inductive steps are for \ref{eqASPMLTrans9} which we prove separately) where $H(r) = \textit{occurred(e, In, I)}$.  For \ref{eqASPSemTrans11} - \ref{eqASPSemTrans14} if $M_P \models \asp{occurred(}p\asp{,}\textit{In}^{i}\asp{,}j\asp{)}$ where $p = a$ for \ref{eqASPSemTrans11} and \ref{eqASPSemTrans14} and $p = d$ for \ref{eqASPSemTrans12} and \ref{eqASPSemTrans13} given that $p \in E^{i}_{j}$ then assume by the inductive hypothesis that $p \in \textit{GR}^{i}(S^{i}_{j}, \{ \textit{se}^{i}_{j} \})$, therefore $e \in \textit{GR}^{i}(S^{i}_{j}, \{ \textit{se}^{i}_{j} \})$ 
\item By 2.2.4.4., 2.2.4.6. and 2.2.4.9. we have shown for each applied rule \ref{eqASPSemTrans11}-\ref{eqASPSemTrans14} such that if by construction $e \in E^{i}_{j}$ then we have the necessary conditions for $e^{\prime} \in \textit{GR}^{i}(S^{i}_{j}, \{ \textit{se}^{i}_{j} \})$.
\end{enumerate}
\item \ref{eqASPMLTrans9} - 
\begin{enumerate}[label*=\arabic*.]
\item If a rule $r$ generated by the transformation \ref{eqASPMLTrans9} is applied then we have $M_P \models \asp{occurred(} e^{\prime}\asp{, }\textit{In}^i \asp{,} j \asp{)}$ and by construction of $E^{i}_{j}$ we have $e^{\prime} \in E^{i}_{j}$. 
\item If $r$ is applied we  must also have $M_P \models \asp{holdsat(pow(}e^{\prime}\asp{),} \textit{In}^{i}\asp{, }j \asp{),}$ and $M_P \models \textit{EX(X,} \pazocal{I}^i)$, and by construction of $S^{i}_{j}$ that $S^{i}_{j} \models \asp{pow(}e^{\prime}\asp{),}$ and $S^{i}_{j} \models X$. 
\item If $r$ is applied then $M_P \models \asp{occurred(} e\asp{, }\textit{In}^i \asp{,} j \asp{)}$ which depends recursively on another applied rule. The base cases are \ref{eqASPSemTrans3}-\ref{eqASPSemTrans5} \ref{eqASPSemTrans11}-\ref{eqASPSemTrans14} (proven). If there is an applied rule $r \in \Pi^{\pazocal{ML}(k)}$ such that $H(r) = M_P \models \asp{occurred(}e\asp{,}\textit{In}^{i}\asp{,}j\asp{)}$ for some $e$ then by construction of $E^{i}_{j}$ we have $e \in E^{i}_{j}$. The inductive hypothesis is that $e \in  \textit{GR}^{i}(S^{i}_{j}, \{ \textit{se}^{i}_{j} \})$. We assume by the inductive hypothesis that if \ref{eqASPMLTrans9} is applied then $M_P \models \asp{occurred(} e\asp{, }\textit{In}^i \asp{,} j \asp{)}$, by construction $e \in E^{i}_{j}$ and thus $e \in \textit{GR}^{i}(S^{i}_{j}, \{ \textit{se}^{i}_{j} \})$. 
\item By 2.2.5.1. 2.2.5.2. and 2.2.5.3. and \ref{eqGR4} if $r$ is applied then $e^{\prime} \in \textit{GR}^{i}(S^{i}_{j}, \{ \textit{se}^{i}_{j} \})$.
\item Thus if a rule produced by \ref{eqASPMLTrans9} is applied then $e^{\prime} \in \textit{GR}^{i}(S^{i}_{j}, \{ \textit{se}^{i}_{j} \})$.
\end{enumerate}
\item \ref{eqASPMLTrans14} -
\begin{enumerate}[label*=\arabic*.]
\item If a rule $r$ generated by the transformation \ref{eqASPMLTrans14} is applied then we have $M_P \models \asp{occurred(} e^{\prime}\asp{, }\textit{In}^i \asp{,} j \asp{)}$ and by construction of $E^{i}_{j}$ we have $e^{\prime} \in E^{i}_{j}$. 
\item If $r$ is applied we  must also have for some $\langle h, i \rangle \in R, e \in \pazocal{E}^{h}_{\textit{norm}} \cap \pazocal{E}^{i}_{\textit{norm}}$
\item We also have that $M_P \models \asp{occurred(} e\asp{, }\textit{In}^h \asp{,} j \asp{)}$ which depends recursively on another applied rule. The base cases are \ref{eqASPSemTrans3}-\ref{eqASPSemTrans5} \ref{eqASPSemTrans11}-\ref{eqASPSemTrans14} (proven). The inductive hypothesis is that if there is an applied rule $r \in \Pi^{\pazocal{ML}(k)}$ such that $H(r) = \asp{occurred(}e\asp{,}\textit{In}^{h}\asp{,}j\asp{)}$ for some $e$, by construction of $E^{h}_{j}$ we have $e \in E^{h}_{j}$, then we have $e \in \textit{GR}^{h}(S^{h}_{j}, \{ \textit{se}^{h}_{j} \})$. We assume by the inductive hypothesis that if \ref{eqASPMLTrans14} is applied then $M_P \models \asp{occurred(} e\asp{, }\textit{In}^h \asp{,} j \asp{)}$, by construction $e \in E^{h}_{j}$ and thus \\$e \in \textit{GR}^{h}(S^{i}_{j}, \{ \textit{se}^{h}_{j} \})$.
\item Thus by 2.2.6.2., 2.2.6.3. and by \ref{eqGR9} $e^{\prime} \in \textit{GR}^{i}(S^{i}_{j}, \{ \textit{se}^{i}_{j} \})$. 
\item Thus, if a rule produced by \ref{eqASPMLTrans14} is applied then $e^{\prime} \in \textit{GR}^{i}(S^{i}_{j}, \{ \textit{se}^{i}_{j} \})$.
\end{enumerate}
\end{enumerate}
We have proven that under the assumption that $e^{\prime} \in E^{i}_{j}$ then $e^{\prime} \in \textit{GR}^{i}(S^{i}_{j}, \{ \textit{se}^{i}_{j} \})$ and thus $E^{i}_{j} \subseteq \textit{GR}^{i}(S^{i}_{j}, \{ \textit{se}^{i}_{j} \})$.
\end{enumerate}
We have proven $E^{i}_{j} \subseteq \textit{GR}^{i}(S^{i}_{j}, \{ \textit{se}^{i}_{j} \})$ and $\textit{GR}^{i}(S^{i}_{j}, \{ \textit{se}^{i}_{j} \}) \subseteq E^{i}_{j}$ therefore $E^{i}_{j} = \textit{GR}^{i}(S^{i}_{j}, \{ \textit{se}^{i}_{j} \})$.
\item $\forall i \in [1, n], \forall j \in [1,k] : S^{i}_j = \textit{TR}^{i}(S^{i}_{j-1}, E^{i}_{j})$ - by Definition~\ref{defST}:
\begin{enumerate}[label*=\arabic*.]
\item By definition~\ref{defST} We need to show that \\$f \in (S^{i}_{j} \cap \pazocal{F}^{i}_{\textit{inert}}) \backslash \textit{TERM}^{i}(S^{i}_{j}, E^{i}_{j}) \cup \textit{INIT}^{i}(S^{i}_{j}, E^{i}_{j})$ or $\exists \langle h, i \rangle \in R, f \in (\pazocal{F}^{h}_{\textit{cnorm}} \cup \pazocal{F}^{h}_{\textit{anorm}}) \cap$ \\ $ \pazocal{F}^{i}_{\textit{ninert}} : f \in S^{h}_{j}$ or $f \in \textit{FD}^{i}(S^{i}_j)$ or $f in \overline{\textit{DC}}^{i}(S^{i}_j)$ iff $f \in S^{i}_{j}$.
\item We will first show $f \in (S^{i}_{j} \cap \pazocal{F}^{i}_{\textit{inert}}) \backslash \textit{TERM}^{i}(S^{i}_{j}, E^{i}_{j}) \cup \textit{INIT}^{i}(S^{i}_{j}, E^{i}_{j})$ iff $f \in S^{i}_{j}$.
\begin{enumerate}[label*=\arabic*.]
\item We will show $f \not \in \textit{TERM}^{i}(S^{i}_{j-1}, E^{i}_{j-1})$ iff \\$M_P \not \models \asp{terminated(}f\asp{,}\textit{In}^{i}\asp{,}j-1\asp{)}$. We will show by contraposition $M_P \models \asp{terminated(}f\asp{,}\textit{In}^{i}\asp{,}j-1\asp{)}$ iff there is an applied rule $r \in P^{*}$ such that $H(r) = \asp{terminated(}f\asp{,}\textit{In}^{i}\asp{,}j-1\asp{)}$. Therefore we will show a rule of the type \ref{eqASPMLTrans7} or \ref{eqASPSemTrans15} with $\asp{terminated(}f\asp{,}\textit{In}^{i}\asp{,}j-1\asp{)}$ in the head is applied if and only if $f \in \textit{TERM}^{i}(S^{i}_{j-1}, E^{i}_{j-1})$.
\begin{enumerate}[label*=\arabic*.]
\item We will show \ref{eqASPMLTrans7} produces an applied rule $r$ such that $H(r) = \asp{terminated(}f\asp{,}\textit{In}^{i}\asp{,}j-1\asp{)}$ iff  we have all the conditions of \ref{eqFIT21}. The rule $r$ is applied such that $M_P \models  \asp{occurred(} e\asp{,} \textit{In}^i\asp{,} j-1 \asp{)}$, $M_P \models \textit{EX(X,} \pazocal{I}^i)$, $M_P \models \asp{holdsat(}f\asp{,} \textit{In}^{i}\asp{,} j-1 \asp{)}$, $M_P \models \asp{instant(}j-1\asp{)}$ iff $f \in \pazocal{C}^{i\downarrow}(X,e)$. Thus by construction we have $S^{i}_{j-1} \models X$, $S^{i}_{j-1} \models f$ and $e \in E^{i}_{j-1}$. Therefore a rule $r$ produced by the transformation \ref{eqASPMLTrans7} is applied iff  we have all the conditions of \ref{eqFIT21}.
\item We will show the rule $r$ in \ref{eqASPSemTrans15} is applied such that \\$H(r) = \asp{terminated(}f\asp{,}\textit{In}^{i}\asp{,}j-1\asp{)}$ iff we have all the conditions of \ref{eqFIT22}. The rule $r$ is applied such that $M_P \models \asp{occurred(viol}f\asp{),} \textit{In}^i\asp{,} j-1 \asp{)}$ or $M_P \models \asp{occurred(disch}f\asp{),} \textit{In}^i\asp{,} j-1 \asp{)}$, and $M_P \models \asp{holdsat(}f\asp{,} \textit{In}^{i}\asp{,} j-1 \asp{)}$. Thus $r$ is applied iff by construction we have $S^{i}_{j-1} \models X$, $S^{i}_{j-1} \models f$, and $\textit{disch}(f) \in E^{i}_{j-1}$ or $\textit{viol}(f) \in E^{i}_{j-1}$. Therefore the rule \ref{eqASPSemTrans15} is applied iff we have all the conditions of \ref{eqFIT22}.
\item Therefore a rule produced by \ref{eqASPMLTrans7} or the rule \ref{eqASPSemTrans15} is applied such that $H(r) = \asp{terminated(}f\asp{,}\textit{In}^{i}\asp{,}j-1\asp{)}$ iff \ref{eqFIT21} or \ref{eqFIT22} are met iff $f \in \textit{TERM}^{i}(S^{i}_{j-1}, E^{i}_{j-1})$.
\item By 3.1.1.1. - 3.1.1.3. a rule $r$ of type \ref{eqASPMLTrans7} or \ref{eqASPSemTrans15} is applied with $H(r) = \asp{terminated(}f\asp{,}\textit{In}^{i}\asp{,}j\asp{)}$ iff we have the conditions of \ref{eqFIT21} or \ref{eqFIT22} iff \\ $f \in \textit{TERM}^{i}(S^{i}_{j-1}, E^{i}_{j-1})$.
\end{enumerate}
By contraposition we have shown $\forall h \in [1,n] : f \not \in \textit{TERM}^{i}(S^{i}_{j-1}, E^{i}_{j-1})$ iff \\$M_P \not \models \asp{terminated(}f\asp{,}\textit{In}^{i}\asp{,}j-1\asp{)}$.
\item We will show that $f \in \textit{INIT}^{i}(S^{i}_{j-1}, E^{i}_{j-1})$ iff \\$M_P \models \asp{initiated(}f\asp{,}\textit{In}^{i}\asp{,}j-1\asp{)}$. We have $M_P \models \asp{initiated(}f\asp{,}\textit{In}^{i}\asp{,}j-1\asp{)}$ iff there is an applied rule $r \in P^{*}$ such that $H(r) = \asp{initiated(}f\asp{,}\textit{In}^{i}\asp{,}j-1\asp{)}$ iff the rule $r$ is from the transformation \ref{eqASPMLTrans6}.
\begin{enumerate}[label*=\arabic*.]
\item We will show \ref{eqASPMLTrans6} produces an applied rule $r$ such that $H(r) = \asp{initiated(}f\asp{,}\textit{In}^{i}\asp{,}j-1\asp{)}$ iff we have all the conditions of \ref{eqFIT11}. According to \ref{eqASPMLTrans6} an applied rule $r$ is produced iff  $M_P \models \asp{occurred(} e\asp{, } \textit{In}^i \asp{,} j-1\asp{)}$ and $M_P \models \textit{EX(X,} \pazocal{I}^i)$ and $f \in \pazocal{C}^{i\uparrow}(X,e)$ iff by construction we have $e \in E^{i}_{j-1}$ and $S^{i}_{j-1} \models X$. Therefore the rule $r$ produced by the transformation \ref{eqASPMLTrans6} is applied iff we have all the conditions of \ref{eqFIT11} s.t. $f \in \textit{INIT}(S^{i}_{j-1}, E^{i}_{j-1})$.
\end{enumerate}
We have shown $f \in \textit{INIT}^{i}(S^{i}_{j-1}, E^{i}_{j-1})$ iff $M_P \models \asp{initiated(}f\asp{,}\textit{In}^{i}\asp{,}j-1\asp{)}$.
\item We have shown $\forall h \in [1,n] : f \not \in \textit{TERM}^{i}(S^{i}_{j-1}, E^{i}_{j-1})$ iff \\$M_P \not \models \asp{terminated(}f\asp{,}\textit{In}^{i}\asp{,}j-1\asp{)}$ and \\ $f \in \textit{INIT}^{i}(S^{i}_{j-1}, E^{i}_{j-1})$ iff $M_P \models \asp{initiated(}f\asp{,}\textit{In}^{i}\asp{,}j-1\asp{)}$.
\item The rule $r$ in \ref{eqASPSemTrans1} where \\ $H(r) = \asp{holdsat(}f\asp{,} \textit{In}^{i}\asp{,} j \asp{)}$ such that\\$M_P \models \asp{ifluent(}f, \textit{In}^{i}\asp{)}$ iff \\$f \not \in \textit{TERM}^{i}(S^{i}_{j-1}, E^{i}_{j-1})$ iff by construction $S^{i}_{j} \models f$ and \ref{eqASPMLTrans4} $f \in \pazocal{F}^{i}_{\textit{inert}}$.
\item By 3.2.1. the rule $r$ in \ref{eqASPSemTrans1} is applied iff \\$f \in S^{i}_{j-1} \cap \pazocal{F}^{i}_{\textit{inert}} \wedge f \not \in \textit{TERM}^{i}(S^{i}_{j-1}, E^{i})$ and therefore iff we have all the conditions in \ref{eqST11}.
\item By 3.2.2. the rule $r$ in \ref{eqASPSemTrans2} is applied where $H(r) = \asp{holdsat(}f\asp{,} \textit{In}^{i}\asp{,} j \asp{)}$, iff $M_P \models \asp{ifluent(}f, \textit{In}^{i}\asp{)}$, $f \in \textit{INIT}^{i}(S^{i}_{j-1}, E^{i}_{j-1})$ and $f \not \in \textit{TERM}^{i}(S^{i}_{j-1}, E^{i}_{j-1})$ iff $f \in \textit{INIT}^{i}(S^{i}_{j-1}, E^{i}) \wedge f \not \in \textit{TERM}^{i}(S^{i}_{j-1}, E^{i})$ and therefore iff we have all the conditions in \ref{eqST12}. 
\end{enumerate}
We have shown $f \in (S^{i}_{j} \cap \pazocal{F}^{i}_{\textit{inert}}) \backslash \textit{TERM}^{i}(S^{i}_{j}, E^{i}_{j}) \cup \textit{INIT}^{i}(S^{i}_{j}, E^{i}_{j})$ iff by construction $f \in S^{i}_{j}$.
\item We will now show $\exists \langle h, i \rangle \in R, n \in (\pazocal{F}^{h}_{\textit{cnorm}} \cup \pazocal{F}^{h}_{\textit{anorm}}) \cap \pazocal{F}^{i}_{\textit{ninert}} : n \in S^{h}_{0} \Rightarrow n \in S^{i}_{0}$ iff $f \in S^{i}_{j}$:
\begin{enumerate}[label*=\arabic*.]
\item According to \ref{eqASPMLTrans13} we have an AnsProlog rule \\$r = \asp{holdsat(} n \asp{, }\textit{In}^i \asp{, I) :- } \asp{holdsat(} n\asp{, }\textit{In}^h\asp{, I).}$
\item By 1.2.1. and construction of $S^{h}_{0}$ we have $M_P \models \asp{holdsat(} n\asp{, }\textit{In}^h\asp{, I)}$.
\item By \ref{eqASPSemTrans16} we have $\asp{instant(}j\asp{)}. \in \Pi^{\pazocal{ML}(k)}$, a fact and therefore $M_P \models \asp{instant(}j\asp{)}$ and thus $r$ is grounded s.t. \\$r = \asp{holdsat(} n \asp{, }\textit{In}^i \asp{, }j\asp{) :- }$ \\ $\asp{holdsat(} n\asp{, }\textit{In}^h\asp{, }j\asp{).} \in \Pi^{*}$.
\item By 3.3.2. and 3.3.3. $\forall l \in B(r^{\prime}) : M_P \models l$, therefore $M_P \models H(r^{\prime})$ and by construction of $S^{i}_{0}$ we have $f \in S^{i}_{j}$.
\end{enumerate}
We have shown $\exists \langle h, i \rangle \in R, n \in (\pazocal{F}^{h}_{\textit{cnorm}} \cup \pazocal{F}^{h}_{\textit{anorm}}) \cap \pazocal{F}^{i}_{\textit{ninert}} : n \in S^{h}_{0} \Rightarrow n \in S^{i}_{0}$ iff by construction $f \in S^{i}_{j}$.
\item We will now show $f \in \textit{FD}^{i}(S^{i}_{j})$ iff $f \in S^{i}_j$.
\begin{enumerate}
\item By \ref{eqDepFl1} and construction $S^{i}_j \subseteq \textit{FD}^{i}(S^{i}_j)$.
\item By \ref{eqDepFl2} if $\exists X \in \pazocal{X}, f \in S^{i}_j, f^{\prime} \in \pazocal{D}^{i}(X, f) : S^{i}_j \models X$ then $f^{\prime} \in S^{i}_j$.
\item By 3.4.ii and \ref{eqASPMLTrans12} we have an AnsProlog rule $r = \asp{holdsat(} f^{\prime}\asp{, }\textit{In}^i \asp{, I) :- } \\
\asp{holdsat(} f\asp{, }\textit{In}^i\asp{, I),} \; \textit{EX(X,} \pazocal{I}^i), \asp{instant(I).}$.
\item By  \ref{eqASPSemTrans16} we have $\asp{instant(}j\asp{)}. \in \Pi^{\pazocal{ML}(k)}$, a fact and therefore $M_P \models \asp{instant(}j\asp{)}$ and thus $r$ is grounded s.t. \\$r = \asp{holdsat(} f^{\prime}\asp{, }\textit{In}^i \asp{, }j\asp{) :- }$ \\ $\asp{holdsat(} f\asp{, }\textit{In}^i\asp{, }j\asp{),} \; \textit{EX(X,} \pazocal{I}^i), \asp{instant(}j\asp{).} \in \Pi^{*}$.
\item By 3.4.iii and construction of $S^{i}_j$ we have $M_P \models \textit{EX(X,} \pazocal{I}^i)$ and $M_P \models \asp{holdsat(} f\asp{, }\textit{In}^i\asp{, }j\asp{)}$.
\item By 3.4.iii, 3.4.iv and 3.4.v we have $\forall l \in B(r) : M_P \models l$, therefore $M_P \models H(r)$ and by construction of $S^{i}_{j}$ we have $f^{\prime} \in S^{i}_{j}$.
\end{enumerate}
We have shown $f \in \textit{FD}^{i}(S^{i}_{j})$ iff $f \in S^{i}_j$.
\item By Lemma~\ref{theoremAbstraction} we have $S^{i}_{0} = \overline{\textit{DC}}^{i}(S^{i}_{0})$.
\item By 3.2., 3.3., 3.4. and 3.5. we have proven $f \in (S^{i}_{j} \cap \pazocal{F}^{i}_{\textit{inert}}) \backslash \textit{TERM}^{i}(S^{i}_{j}, E^{i}_{j}) \cup \textit{INIT}^{i}(S^{i}_{j}, E^{i}_{j})$ or $\exists \langle h, i \rangle \in R, f \in (\pazocal{F}^{h}_{\textit{cnorm}} \cup \pazocal{F}^{h}_{\textit{anorm}}) \cap \pazocal{F}^{i}_{\textit{ninert}} : f \in S^{h}_{j}$ or $f \in \textit{FD}^{i}(S^{i}_j)$ or $f in \overline{\textit{DC}}^{i}(S^{i}_j)$ iff $f \in S^{i}_{j}$. 
\end{enumerate}
We have proven $\forall i \in [1, n], \forall j \in [1,k] : S^{i}_j = \textit{TR}^{i}(S^{i}_{j-1}, E^{i}_{j})$.
\end{enumerate}
We have proven a) $\forall i \in [1, n] : S^{i}_0 \subseteq \Delta^{i}$, $\exists \langle h, i \rangle \in R, n \in (\pazocal{F}^{h}_{\textit{cnorm}} \cup \pazocal{F}^{h}_{\textit{anorm}}) \cap \pazocal{F}^{i}_{\textit{ninert}} : n \in S^{h}_{0} \Rightarrow n \in S^{i}_{0}$, $\forall i \in [1,n] : S^{i}_0 = \textit{FD}^{i}(S^{i}_0)$ and $\forall i \in [1,n] : S^{i}_0 = \overline{\textit{DC}}^{i}(S^{i}_0)$. b) $\forall i \in [1, n], \forall j \in [1,k] : E^{i}_j = \textit{GR}^{i}(S^{i}_{j-1}, \{ \textit{se}^{i}_{j} \})$. Where $\textit{GR}^{i}$ is the event generation operation for an institution $\pazocal{I}^{i}$  w.r.t. $E = \langle E^{1}_{j}, ..., E^{n}_{j}\rangle$. c) $\forall i \in [1, n], \forall j \in [1,k+1] : S^{i}_j = \textit{TR}^{i}(S^{i}_{j-1}, E^{i}_{j})$. Where $\textit{TR}^{i}$ is the state transition operation for an institution $\pazocal{I}^{i}$  w.r.t. $S = \langle S^{1}_{j}, ..., S^{n}_{j}\rangle$. Therefore we have proven $M$ is the model of $\pazocal{ML}$ w.r.t. $\textit{ctr}$.
\end{proof}

\subsection{Completeness Proof} 
\label{proofCompl}

To prove completeness we take the same approach as in \cite[p. 161]{Cliffe2007}.

\begin{proof}{\textbf{Theorem~\ref{theorCompl} Completeness}} We need to show that $M_P$ is a model for $P^{*}$ and also a \textit{minimal} model for $P^{*}$. We show the interpretation $M_P$ is a model for the reduct of $P^{*, M_P}$ of $P^{*}$ w.r.t $M_P$. Let $r \in P^{*, M_P}$ be an applicable rule. We need to show that $M_P \models \textit{H}(r)$, that the rule is applied. Each type of rule from Definition~\ref{defASPMLTrans}, Definition~\ref{defASPDCATrans}, Definition~\ref{defASPCompTraceTrans} and Definition~\ref{defASPMLSemTrans} is addressed.
\begin{itemize}
\item \textit{r} is a fact of type \ref{eqASPMLTrans1}-\ref{eqASPMLTrans5} or a fact in \ref{eqASPSemTrans16}. True by construction of $M_P$.
\item \textit{r} is of type \ref{eqASPSemTrans1} -  by the reduct we know $\asp{terminated(}f, \textit{In}^{i}, j\asp{)}$ is false. By \ref{eqThCo4} for $f$ at $j$ we know $f \in S^{i}_{j}$ and by \ref{eqThCo1} $M_P \models \asp{holdsat(}f, \textit{In}^{i}, j\asp{)}$.
\item \textit{r} is of type \ref{eqASPSemTrans2} -  $\asp{initiated(}f, \textit{In}^{i}, j\asp{)}$ since $f \in S^{i}_{j}$ and $f \not \in S^{i}_{j-1}$ by \ref{eqThCo3}. By \ref{eqThCo3} and \ref{eqThCo1} $M_P \models \asp{holdsat(}f, \textit{In}^{i}, j\asp{)}$.
\item \textit{r} is of type \ref{eqASPSemTrans3} - from the way $\asp{instant(}j)$ is created in \ref{eqThCo13} we can infer that $\exists j \in [k] : E^{i}_{j}$. From \ref{eqGR10} and \ref{eqThCo6} we infer $M_P \models \asp{occurred(now}, \textit{In}^{i}, j)$.
\item \textit{r} is of type \ref{eqASPSemTrans4} - we know $\asp{observed}(e_{\textit{obs}}, \textit{In}^{i}, j)$ atoms originate from the composite trace \textit{ctr}. Given that $M_P \models \asp{evtype}(e_{\textit{obs}}, \textit{In}^{i}, \asp{ex})$ by \ref{eqThCo9} we have $e_\textit{obs} \in \pazocal{E}^{i}_{\textit{obs}}$ and by \ref{defSynchTrace} we have a synchronised trace $\textit{str}^{i} = \langle e_0, ..., e_k \rangle $ for $\pazocal{I}^{i}$ where $e_j = e_{\textit{obs}}$. Therefore by the definition of a multi-level governance institution model \ref{defMLGModel} and by \ref{eqGR11} we know $e_{\textit{obs}} \in E^{i}_{j}$. Therefore by \ref{eqThCo6} $M_P \models \asp{occurred}(e_{\textit{obs}}, \textit{In}^{i}, j)$.
\item \textit{r} is of type \ref{eqASPSemTrans5} - we know $\asp{observed}(e_{\textit{obs}}, \textit{In}^{i}, j)$ atoms originate from the composite trace \textit{ctr}. By the reduct we know $\asp{evtype}(e_{\textit{obs}}, \textit{In}^{i}, \asp{ex})$ is not true, this implies by \ref{eqThCo9} $e_\textit{obs} \not \in \pazocal{E}^{i}_{\textit{obs}}$ and by \ref{defSynchTrace} we have a synchronised trace $\textit{str}^{i} = \langle e_0, ..., e_k \rangle $ for $\pazocal{I}^{i}$ where $e_j = e_{\textit{null}}$. Therefore by \ref{eqThCo7} we have $M_P \models \asp{occurred}(\asp{null}, \textit{In}^{i}, j)$.
\item \textit{r} is of type \ref{eqASPSemTrans6} - always true.
\item \textit{r} is of type \ref{eqASPSemTrans7} - true by structure of \textit{ctr} and \ref{eqThCo5}.
\item \textit{r} is of type \ref{eqASPSemTrans8}, \ref{eqASPSemTrans9} or \ref{eqASPSemTrans10} - true by \ref{eqThCo5}.
\item \textit{r} is of type \ref{eqASPSemTrans11} or \ref{eqASPSemTrans13} - by construction this implies $e \in E^{i}_{j}$ or $e \in S^{i}_{j}$, and by \ref{eqASPSemTrans11} $\textit{obl}(e, d) \in S^{i}_{j}$ or by \ref{eqASPSemTrans13}  $\textit{pro}(a, e) \in S^{i}_{j}$. Therefore by \ref{eqGR14} or \ref{eqGR16} we have $\textit{disch}(\textit{obl}(e, d)) \in E^{i}_{j}$ or $\textit{disch}(\textit{pro}(a, e)) \in E^{i}_{j}$ and thus $M_P \models H(r)$.
\item \textit{r} is of type \ref{eqASPSemTrans12} or \ref{eqASPSemTrans14} - similar to the previous case, by construction this implies $e \in E^{i}_{j}$ or $e \in S^{i}_{j}$, and by \ref{eqASPSemTrans12} $\textit{obl}(a, e) \in S^{i}_{j}$ or by \ref{eqASPSemTrans14}  $\textit{pro}(e, d) \in S^{i}_{j}$. By the reduct and construction of $E^{i}_{j}$ we know $\textit{disch}(\textit{obl}(e, d)) \not \in E^{i}_{j}$ by \ref{eqASPSemTrans12} or $\textit{disch}(\textit{pro}(a, e)) \in E^{i}_{j}$ by \ref{eqASPSemTrans14}. Therefore by \ref{eqGR15} or \ref{eqGR17} we have $\textit{viol}(\textit{obl}(a, e)) \in E^{i}_{j}$ or $\textit{viol}(\textit{pro}(e, d)) \in E^{i}_{j}$ and thus $M_P \models H(r)$.
\item \textit{r} is of type \ref{eqASPSemTrans15} - by construction we know $N \in S^{i}_{j}$ and $\textit{disch}(N) \in E^{i}_{j}$ or $\textit{viol}(N) \in E^{i}_{j}$ and by \ref{eqASPMLTrans4} $N \in \pazocal{F}^{i}_{\textit{inert}}$. Therefore we have the conditions for $N \in S^{i}_{j} \backslash S^{i}_{j+1} \cap \pazocal{F}^{i}_{\textit{inert}}$ by \ref{eqFIT22}, \ref{eqST11} or \ref{eqST12}, and \ref{eqMLGM4}. Thus by \ref{eqThCo4} we have $M_P \models H(r)$.
\item \textit{r} is of type \ref{eqASPSemTrans16} where $H(r)$ is a \asp{next/2} atom - $M_P \models H(r)$ by \ref{eqThCo13} and \ref{eqThCo15}.
\item \textit{r} is of type \ref{eqASPMLTrans6} - from the creation of the rule and the fact that the body elements are true we infer $f \in \pazocal{F}^{i}_{\textit{inert}}$ and by \ref{eqThCo1} $S^{i}_{j} \models X$, by \ref{eqThCo6} that $e \in E^{i}_{j}$ and $f \in \pazocal{C}^{\i \uparrow}(X, e)$. By $M$ being a model and by \ref{eqFIT11} we have the conditions for $f \in \textit{INIT}(S^{i}_{j}, E^{i}_{j})$. By the reduct we know $S^{i}_{j-1} \not \models f$ and by \ref{eqMLGM4}, \ref{eqST12} we have $S^{i}_{j} \models f$. Therefore we have all the conditions for $M_P \models H(r)$ by \ref{eqThCo3}.
\item \textit{r} is of type \ref{eqASPMLTrans7} - from the creation of the rule and the fact that the body elements are true we infer $f \in \pazocal{F}^{i}_{\textit{inert}}$ and by \ref{eqThCo1} $S^{i}_{j} \models X$ and $S^{i}_{j} \models f$, by \ref{eqThCo6} that $e \in E^{i}_{j}$ and $f \in \pazocal{C}^{i \downarrow}(X, e)$. By $M$ being a model and by \ref{eqFIT11} we have the conditions for $f \in \textit{TERM}(S^{i}_{j}, E^{i}_{j})$. By \ref{eqMLGM4} and \ref{eqST11} we have $S^{i}_{j + 1} \not \models f$. Therefore we have all the conditions for $M_P \models H(r)$ by \ref{eqThCo4}.
\item \textit{r} is of type \ref{eqASPMLTrans9} - from the creation of the rule and the fact that the body elements are true we infer $S^{i}_{j} \models X$, $S^{i}_{j} \models \textit{pow}(e^{\prime})$, $e \in E^{i}_{j}$  and $e^{\prime} \in \pazocal{G}^{i}(X, e)$. By $M$ being a model and by \ref{eqGR13}  we have the conditions for $e^{\prime} \in E^{i}_{j}$. Therefore we have all the conditions for $M_P \models H(r)$ by \ref{eqThCo2}.
\item \textit{r} is of type \ref{eqASPMLTrans12} - from the creation of the rule and $\pazocal{D}^{i}$ in definition~\ref{def:inst} we infer that $f^{\prime} \in \pazocal{F}^{i}_{\textit{ninert}}$, $S^{i}_{j} \models X$ and $S^{i}_{j} \models f$. We have all the conditions such that by $M$ being a model and \ref{eqDepFl2} we conclude $M_P \models H(r)$ by \ref{eqThCo1}.
\item \textit{r} is of type \ref{eqASPMLTrans10} - from the creation of the rule we infer $f \in \Delta^{i}$. By Definition~\ref{defMLGModel} and \ref{eqIS1} and since $\overline{\textit{DC}}^{i}$ is monotonic we infer that $f \in S^{i}_{0}$. Therefore by \ref{eqThCo14} and \ref{eqThCo1} we have $M_P \models H(r)$.
\item \textit{r} is of type \ref{eqASPMLTrans13} - from the creation of the rule we infer that $f^{\prime} \in \pazocal{F}^{i}_{\textit{ninert}}$ and $\langle h, i \rangle \in R$. By the rule being applied we infer that $S^{h}_{j} \models f$ and $S^{i}_{j} \models f$. We have all the conditions such that by $M$ being a model and \ref{eqST13} we conclude $M_P \models H(r)$.
\item \textit{r} is of type \ref{eqASPMLTrans14} - from the creation of the rule we infer that $e^{\prime} \in \pazocal{E}^{i}_{\textit{norm}}$ and $\langle h, i \rangle \in R$. By the rule being applied we infer that $e \in E^{h}_{j}$ and $e \in E^{i}_{j}$. We have all the conditions such that by $M$ being a model and \ref{eqGR18} we conclude $M_P \models H(r)$.
\item \textit{r} is of type \ref{eqASPMLTrans11} - from the creation of the rule this implies $f \equiv f^{\prime}$, by Definition\ref{defStateForm} $S^{i}_{j} \models f$ and by \ref{eqThCo1} $M_P \models H(r)$.
\item \textit{r} is of type \ref{eqASPDCATrans1}, \ref{eqASPDCATrans2}, \ref{eqASPDCATrans5}, \ref{eqASPDCATrans6}, \ref{eqASPDCATrans3}, \ref{eqASPDCATrans4}, - we will first show by induction that for a rule $r^{\prime}$ of these types such that $r^{\prime} = \asp{holdsat}(n^{\prime}, \textit{In}^{i}, j) \asp{:-}$ \\ $\textit{CN}, C, \asp{nifluent(}n^{\prime}, \textit{In}^{i} \asp{),} \asp{holdsat}(\textit{pow}(b), \textit{In}^{i}, j), \asp{instant(I).}$, if $\exists \textit{EX(n)} \asp{:} \textit{EX}(X, \pazocal{I}^{i})\asp{;} \in \textit{CN} : M_P \models \textit{EX}(X, \pazocal{I}^{i})$  then $\langle N, n^{\prime} \rangle \in \textit{DC}^{i}(S^{i}_{j})$ such that $n \in N$. We will then show that the rule $r$ being applied means that $n^{\prime} \in \overline{\textit{DC}}^{i}(S^{i}_{j})$ and consequently $M_P \models H(r)$.
\begin{enumerate}[label*=\arabic*.]
\item First, by induction on two counters:
\begin{enumerate}[label*=\arabic*.]
\item \textbf{Base case 1:} \ref{eqASPDCATrans1} and \ref{eqASPDCATrans5} -
\begin{enumerate}[label*=\arabic*.]
\item The transformations \ref{eqASPDCATrans1} and \ref{eqASPDCATrans5} gives $r^{\prime} = \asp{holdsat}(n, \textit{In}^{i}, j) \asp{:-}$ \\ $\textit{CN}, C, \asp{holdsat}(\textit{pow}(b), \textit{In}^{i}, j), \\ \asp{nifluent(}n, \textit{In}^{i} \asp{),} \asp{instant(I).}$ or \\$r^{\prime} = \asp{holdsat}(n, \textit{In}^{i}, j) \asp{:-} \textit{CN}, C,\asp{nifluent(}n, \textit{In}^{i} \asp{),} \asp{instant(I).}$ such that $n \in \pazocal{F}^{i}_{\textit{anorm}}$.
\item If $\exists \textit{EX(n)} \asp{:} \textit{EX}(X, \pazocal{I}^{i})\asp{;} \in \textit{CN} : M_P \models \textit{EX}(X, \pazocal{I}^{i})$ then by construction of $S^{i}_{j}$ we know that $S^{i}_{j} \models X$ and if $M_P \models \asp{holdsat}(\textit{pow}(b), \textit{In}^{i}, j)$ then $S^{i}_{j} \models \textit{pow}(a)$.
\item By the creation of $r^{\prime}$ we have $b \in \pazocal{G}^{i}(X, a) \cup \pazocal{D}^{i}(X, a)$ and $a \in \pazocal{E}^{i}_{\textit{inst}} \cup \pazocal{F}^{i}$.
\item Therefore by 1.1.1, 1.1.2, 1.1.3 if $\textit{EX(n)} \asp{:} \textit{EX}(X, \pazocal{I}^{i})\asp{;} \in \textit{CN}, M_P \models \textit{EX}(X, \pazocal{I}^{i})$ then we have all the conditions of \ref{eqDC1} for $\langle N, n^{\prime} \rangle \in \textit{DC}^{i}(S^{i}_{j})$ such that $n \in N$.
\end{enumerate}
\item \textbf{Base case 2:} \ref{eqASPDCATrans2} -
\begin{enumerate}[label*=\arabic*.]
\item The transformations \ref{eqASPDCATrans2} and \ref{eqASPDCATrans6} give us $r^{\prime} = \asp{holdsat}(n, \textit{In}^{i}, j) \asp{:-}$ \\ $\textit{CN}, C, \asp{holdsat}(\textit{pow}(b), \textit{In}^{i}, j), \\ \asp{nifluent(}n, \textit{In}^{i} \asp{),} \asp{instant(I).}$ or \\$r^{\prime} = \asp{holdsat}(n, \textit{In}^{i}, j) \asp{:-} \textit{CN}, C, \asp{nifluent(}n, \textit{In}^{i} \asp{),} \\ \asp{instant(I).}$ such that $n \in \pazocal{F}^{i}_{\textit{anorm}}$. 
\item If $\exists \textit{EX(n)} \asp{:} \textit{EX}(X, \pazocal{I}^{i})\asp{;} \in \textit{CN} : M_P \models \textit{EX}(X, \pazocal{I}^{i})$ then by construction of $S^{i}_{j}$ we know that $S^{i}_{j} \models X$ and if $M_P \models \asp{holdsat}(\textit{pow}(b), \textit{In}^{i}, j)$ then $S^{i}_{j} \models \textit{pow}(a)$.
\item By the creation of $r^{\prime}$ we have $b \in \pazocal{G}^{i}(X, a) \cup \pazocal{D}^{i}(X, a)$ and $a \in \pazocal{E}^{i}_{\textit{inst}} \cup \pazocal{F}^{i}$. \item Therefore by 1.2.1, 1.2.2 and 1.2.3 if $\textit{EX(n)} \asp{:} \textit{EX}(X, \pazocal{I}^{i})\asp{;} \in \textit{CN}, M_P \models \textit{EX}(X, \pazocal{I}^{i})$ then we have all the conditions of \ref{eqDC2} for $\langle N, n^{\prime} \rangle \in \textit{DC}^{i}(S^{i}_{j})$ such that $n \in N$.
\end{enumerate}
\item \textbf{Inductive hypothesis:} - A rule $r^{\prime}$ is of type \ref{eqASPDCATrans1}, \ref{eqASPDCATrans2}, \ref{eqASPDCATrans5}, \ref{eqASPDCATrans6}, \ref{eqASPDCATrans3}, \ref{eqASPDCATrans4} such that $r^{\prime} = \\ \asp{holdsat}(n, \textit{In}^{i}, j) \asp{:-} \textit{CN}, C, \asp{holdsat}(\textit{pow}(b), \textit{In}^{i}, j), \asp{nifluent(}n, \textit{In}^{i} \asp{),} \asp{instant(I).}$ or \\$r^{\prime} =\asp{holdsat}(n, \textit{In}^{i}, j) \asp{:-} \textit{CN}, C, \asp{nifluent(}n, \textit{In}^{i} \asp{),} \asp{instant(I).}$, and $n \in \pazocal{F}^{i}_{\textit{anorm}}$. If $\textit{EX(n)} \asp{:} \textit{EX}(X, \pazocal{I}^{i})\asp{;} \in \textit{CN} : M_P \models \textit{EX}(X, \pazocal{I}^{i})$ then $\langle N, n^{\prime} \rangle \in \textit{DC}^{i}(S^{i}_{j})$ such that $n \in N$.
\item \textbf{Inductive step 1:} \ref{eqASPDCATrans3} -
\begin{enumerate}[label*=\arabic*.]
\item The transformation \ref{eqASPDCATrans3} gives us $r^{\prime \prime} = \asp{holdsat}(\textit{obl}(n^{\prime}, d), \textit{In}^{i}, j) \asp{:-}$ \\ $\textit{CN}^{\prime \prime}, C^{\prime \prime}, \asp{holdsat}(\textit{pow}(b), \textit{In}^{i}, j),$ \\ $\asp{nifluent(}\textit{obl}(n^{\prime}, d), \textit{In}^{i} \asp{),}$ \\ $\asp{instant(I).}$ or \\$r^{\prime \prime} = \asp{holdsat}(\textit{obl}(n^{\prime}, d), \textit{In}^{i}, j) \asp{:-} \textit{CN}^{\prime \prime}, C^{\prime \prime}, \asp{nifluent(}\textit{obl}(n^{\prime}, d), \textit{In}^{i}\asp{),} \asp{instant(I).}$ where \\$\textit{obl}(n^{\prime}, d) \in \pazocal{F}^{i}_{\textit{anorm}}$.
\item We know that $r^{\prime \prime}$ is created conditional on a rule \\$r^{\prime} = \asp{holdsat}(n^{\prime}, \textit{In}^{i}, j) \asp{:-}$ \\ $\textit{CN}^{\prime}, C^{\prime}, \asp{holdsat}(\textit{pow}(b), \textit{In}^{i}, j), \asp{nifluent(}n^{\prime}, \textit{In}^{i} \asp{),} \asp{instant(I).}$ or \\$r^{\prime} = \asp{holdsat}(n^{\prime}, \textit{In}^{i}, j) \asp{:-} \textit{CN}^{\prime}, C^{\prime}, \asp{nifluent(}n^{\prime}, \textit{In}^{i} \asp{),} \asp{instant(I).}$. 
\item By the inductive hypothesis if $\textit{EX(n)} \asp{:} \textit{EX}(X, \pazocal{I}^{i})\asp{;} \in \textit{CN}^{\prime}, M_P \models \textit{EX}(X, \pazocal{I}^{i})$ then $\langle N, n^{\prime} \rangle \in \textit{DC}^{i}(S^{i}_{j})$ such that $n \in N$. 
\item By the creation of $r^{\prime \prime}$ and 3 we know that $\textit{CN}^{\prime \prime}$ is constructed such that $\textit{EX(n)} \asp{:} \textit{EX}(X, \pazocal{I}^{i})\asp{;} \in \textit{CN}^{\prime}, M_P \models \textit{EX}(X, \pazocal{I}^{i})$ iff $\textit{EX(obl(n, d)} \asp{:} \textit{EX}(X, \pazocal{I}^{i})\asp{;} \in \textit{CN}^{\prime \prime}, M_P \models \textit{EX}(X, \pazocal{I}^{i})$. 
\item If $\langle N, n^{\prime} \rangle \in \textit{DC}^{i}(S^{i}_{j})$ then by \ref{eqDC1} $\langle N^{\prime}, \textit{obl}(n^{\prime}, d) \rangle \in \textit{DC}^{i}(S^{i}_{j})$ such that $n \in N$ iff $\textit{obl}(n, d) \in N^{\prime}$.
\item By 1.4.3, 1.4.4 and 1.4.5 if $\textit{EX}(\textit{obl}(n, d)) \asp{:} \textit{EX}(X, \pazocal{I}^{i})\asp{;} \in \textit{CN}^{\prime \prime},$ \\ $M_P \models \textit{EX}(X, \pazocal{I}^{i})$ then $\langle N^{\prime}, \textit{obl}(n^{\prime}, d) \rangle \in \textit{DC}^{i}(S^{i}_{j})$ such that $\textit{obl}(n^{\prime}, d) \in N^{\prime}$.
\end{enumerate}
\item \textbf{Inductive step 2:} \ref{eqASPDCATrans4} -
\begin{enumerate}[label*=\arabic*.]
\item The transformation \ref{eqASPDCATrans4} gives us $r^{\prime \prime} = \asp{holdsat}(\textit{pro}(n^{\prime}, d), \textit{In}^{i}, j) \asp{:-} \\ \textit{CN}^{\prime \prime}, C^{\prime \prime}, \asp{holdsat}(\textit{pow}(b), \textit{In}^{i}, j), \asp{nifluent(}\textit{pro}(n^{\prime}, d), \textit{In}^{i}\asp{),} \asp{instant(I).}$ or \\ $r^{\prime \prime} = \asp{holdsat}(\textit{pro}(n^{\prime}, d), \textit{In}^{i}, j) \asp{:-} \\ \textit{CN}^{\prime \prime}, C^{\prime \prime}, \asp{nifluent(}\textit{pro}(n^{\prime}, d), \textit{In}^{i}\asp{),} \asp{instant(I).}$ where $\textit{pro}(n^{\prime}, d) \in \pazocal{F}^{i}_{\textit{anorm}}$.
\item We know that $r^{\prime \prime}$ is created conditional on rules of the form \\$r^{\prime} = \asp{holdsat}(n^{\prime}, \textit{In}^{i}, j) \asp{:-}$ \\ $\textit{CN}^{\prime}, C^{\prime},$ \\ $\asp{holdsat}(\textit{pow}(b), \textit{In}^{i}, j), \asp{nifluent(}n^{\prime}, \textit{In}^{i} \asp{),} \asp{instant(I).}$ or \\$r^{\prime} = \asp{holdsat}(n^{\prime}, \textit{In}^{i}, j) \asp{:-} \textit{CN}^{\prime}, C^{\prime}, \asp{nifluent(}n^{\prime}, \textit{In}^{i} \asp{),} \asp{instant(I).}$.
\item By the inductive hypothesis for all rules $r^{\prime}$ if $\textit{EX(n)} \asp{:} \textit{EX}(X, \pazocal{I}^{i})\asp{;} \in \textit{CN}^{\prime}, M_P \models \textit{EX}(X, \pazocal{I}^{i})$ then $\langle N, n^{\prime} \rangle \in \textit{DC}^{i}(S^{i}_{j})$ such that $n \in N$. 
\item By the creation of $r^{\prime \prime}$ and 3 we know that $\textit{CN}^{\prime \prime}$ is constructed such that for all rules $r^{\prime}$ we have \\$\textit{EX(n)} \asp{:} \textit{EX}(X, \pazocal{I}^{i})\asp{;} \in \textit{CN}^{\prime}, M_P \models \textit{EX}(X, \pazocal{I}^{i})$ iff $\textit{EX(pro(n, d)} \asp{:} \textit{EX}(X, \pazocal{I}^{i})\asp{;} \in \textit{CN}^{\prime \prime}, M_P \models \textit{EX}(X, \pazocal{I}^{i})$.
\item For all rules $r^{\prime}$ if $\langle N, n^{\prime} \rangle \in \textit{DC}^{i}(S^{i}_{j})$ then by \ref{eqDC2} we have that $\langle N^{\prime}, \textit{pro}(n^{\prime}, d) \rangle \in$ \\ $\textit{DC}^{i}(S^{i}_{j})$ such that $n \in N$ iff $\textit{pro}(n, d) \in N^{\prime}$.
\item By 1.5.3, 1.5.4 and 1.5.5 if $\textit{EX}(\textit{pro}(n, d)) \asp{:} \textit{EX}(X, \pazocal{I}^{i})\asp{;} \in \textit{CN}^{\prime \prime}$ if $M_P \models \textit{EX}(X, \pazocal{I}^{i})$ then $\langle N^{\prime}, \textit{pro}(n^{\prime}, d) \rangle \in \textit{DC}^{i}(S^{i}_{j})$ such that $\textit{pro}(n, d) \in N^{\prime}$.
\end{enumerate}
We have shown by induction that a rule $r^{\prime}$ of type \ref{eqASPDCATrans1}, \ref{eqASPDCATrans2}, \ref{eqASPDCATrans5}, \ref{eqASPDCATrans6}, \ref{eqASPDCATrans3} or \ref{eqASPDCATrans4} such that \\$r^{\prime} = \asp{holdsat}(n^{\prime}, \textit{In}^{i}, j) \asp{:-} \textit{CN}, C, \asp{holdsat}(\textit{pow}(b), \textit{In}^{i}, j), \asp{instant(I).}$ or \\$r^{\prime} = \asp{holdsat}(n^{\prime}, \textit{In}^{i}, j) \asp{:-} \textit{CN}, C, \asp{instant(I).}$, if $\exists \textit{EX(n)} \asp{:} \textit{EX}(X, \pazocal{I}^{i})\asp{;} \in \textit{CN} : M_P \models \textit{EX}(X, \pazocal{I}^{i})$  then $\langle N, n^{\prime} \rangle \in \textit{DC}^{i}(S^{i}_{j})$ such that $n \in N$.
\end{enumerate}
\item We will now show if $r$ of type \ref{eqASPDCATrans1}, \ref{eqASPDCATrans2}, \ref{eqASPDCATrans5}, \ref{eqASPDCATrans6}, \ref{eqASPDCATrans3} or \ref{eqASPDCATrans4} is applied then $n^{\prime} \in \overline{\textit{DC}}^{i}(S^{i}_{j})$ and consequently $M_P \models H(r)$:
\begin{enumerate}[label*=\arabic*.]
\item If $r$ is of type \ref{eqASPDCATrans1}, \ref{eqASPDCATrans2}, \ref{eqASPDCATrans5}, \ref{eqASPDCATrans6} \ref{eqASPDCATrans3} or \ref{eqASPDCATrans4} then \\$r = \asp{holdsat}(n^{\prime}, \textit{In}^{i}, j) \asp{:-} \textit{CN}, C, \asp{holdsat}(\textit{pow}(b), \textit{In}^{i}, j), \asp{instant(I).}$ or \\$r = \asp{holdsat}(n^{\prime}, \textit{In}^{i}, j) \asp{:-} \textit{CN}, C,\asp{instant(I).}$.
\item Under the semantics of aggregates if $r$ is applied then $C$ must be true and $\exists \textit{EX(n)} \asp{:} \textit{EX}(X, \pazocal{I}^{i})\asp{;} \in \textit{CN} : M_P \models \textit{EX}(X, \pazocal{I}^{i})$.
\item By 1 we have for all $\textit{EX(n)} \asp{:} \textit{EX}(X, \pazocal{I}^{i})\asp{;} \in \textit{CN} : M_P \models \textit{EX}(X, \pazocal{I}^{i})$  then $\langle N, n^{\prime} \rangle \in \textit{DC}^{i}(S^{i}_{j})$ such that $n \in N$.
\item Since $r$ is applied we know that $\textit{CN}$ is true, therefore by 2.3. and construction in \ref{eqThCo1} iff $S^{i}_{j} \models N$. Therefore we have $\langle N, n^{\prime} \rangle \in \overline{\textit{DC}}^{i}(S^{i}_{j})$. such that $\forall n \in N : S^{i}_{j} \models n$
\item By Definition~\ref{defDC} we have $n \in \overline{\textit{DC}}^{i}(S^{i}_{j})$, by \ref{eqMLGM2} and \ref{eqIS4} for $j=0$ or \ref{eqMLGM4} and \ref{eqST15} $j \neq 0$ we have $S^{i}_{j} \models n^{\prime}$ and by construction $M_P \models H(r)$.
\end{enumerate}
\end{enumerate}
\end{itemize}
We have shown for every applicable rule $r \in P^{*, M_P}$ that $M_P \models H(r)$ and thus $M_P$ is a model of $P^{*, M_P}$. We will now show that $M_P$ is a \textit{minimal} model of $P^{*, M_P}$ by proving there does not exist a model of $P^{*, M_P}$ that is a strict subset of $M_P$. Let the program $P^{*, M_P \prime}$ be the program comprising all applied rules in $P^{*, M_P}$ stratified into levels $\pi_x$ according to:
\begin{itemize}[label={}]
\item \ref{eqASPMLTrans1} - $\asp{inst(}\textit{In}^i\asp{)} : \pi_0 .$
\item \ref{eqASPMLTrans2} - $\asp{evtype(e,} \textit{In}^i \asp{,ex)} : \pi_0 .$
\item \ref{eqASPMLTrans3} - $\asp{evtype(e,} \textit{In}^i \asp{,inst)} : \pi_0 .$
\item \ref{eqASPMLTrans4} - $\asp{ifluent(f, }\textit{In}^i\asp{)} : \pi_0.$
\item \ref{eqASPMLTrans5} - $\asp{nifluent(f, }\textit{In}^i\asp{)} : \pi_0 .$
\item $\begin{aligned} \text{\ref{eqASPMLTrans6} -} \asp{initiated(} p\asp{, } \textit{In}^i \asp{, J)}: \pi_{3J+2} \asp{:- } & \asp{occurred(} e\asp{, } \textit{In}^i \asp{,} I\asp{)} : \pi_{3J+1}, \\ & \asp{not} \; \asp{holdsat(}p, \textit{In}^{i}, \asp{J)} : \pi_{3J}, \\ &
\textit{EX(X,} \pazocal{I}^J) : \pi_{3J}, \\ \asp{instant(J)} : \pi_0.\end{aligned}$
\item $\begin{aligned} \text{\ref{eqASPMLTrans7} -} \asp{terminated(} p\asp{, }\textit{In}^i \asp{, J)}: \pi_{3J+2} \asp{:- } & \asp{occurred(} e\asp{,} \textit{In}^i\asp{, J)} : \pi_{3J+1}, \\ & 
\textit{EX(X,} \pazocal{I}^i) : \pi_{3J}, \\ & \asp{holdsat(}f\asp{,} \textit{In}^{i}\asp{, J)} : \pi_{3J}, \asp{instant(J)} : \pi_{0}.\end{aligned}$
\item $\begin{aligned} \text{\ref{eqASPMLTrans9} - } \asp{occurred(} e^{\prime}\asp{, }\textit{In}^i \asp{, J)} : \pi_{3J+1} \asp{:- } & \asp{occurred(} e\asp{, }\textit{In}^i\asp{, J)}: \pi_{3J+1}, \asp{holdsat(pow(}e^{\prime}\asp{),} \textit{In}^{i}\asp{, J)} : \pi_{3J}\asp{,} \\ & \textit{EX(X,} \pazocal{I}^i) : \pi_{3J}, \asp{instant(J)} : \pi_{0}. \end{aligned}$
\item $\begin{aligned} \text{\ref{eqASPMLTrans12} - } \asp{holdsat(} f^{\prime}\asp{, }\textit{In}^i \asp{, J) :- } \; \; \asp{holdsat(} f\asp{, }\textit{In}^i\asp{, J),} \; \textit{EX(X,} \pazocal{I}^i), \asp{instant(J).} : \pi_{3J} \end{aligned}$
\item $\text{\ref{eqASPMLTrans10} -} \asp{holdsat(} f\asp{, } \textit{In}^i, \asp{J)} : \pi_{3J} \asp{:-} \asp{start(J)} : \pi_{0} \asp{.}$
\item $\begin{aligned} \text{\ref{eqASPMLTrans13} - } \asp{holdsat(} n \asp{, }\textit{In}^i \asp{, J)} : \pi_{3J} \asp{:-} \asp{holdsat(} n\asp{, }\textit{In}^h\asp{, J).} : \pi_{3J} \end{aligned}$
\item $\begin{aligned} \text{\ref{eqASPMLTrans14} - } \asp{occurred(} e \asp{, }\textit{In}^i \asp{, I)} : \pi_{3J+1} \asp {:- }  \asp{occurred(} e\asp{, }\textit{In}^h\asp{, I).} : \pi_{3J+1} \end{aligned}$
\item $\text{\ref{eqASPMLTrans11} - }\asp{holdsat(} \textit{f}\asp{, } \textit{In}^i, \asp{J)} : \pi_{J} :- \asp{holdsat(} \textit{f}^{\prime}\asp{, } \textit{In}^i, \asp{J)} : \pi_{J} \asp{, } \asp{instant(J)} : \pi_{0}.$
\item $\text{\ref{eqASPDCATrans1} - } \asp{holdsat(obl(}b, d\asp{)}, \textit{In}^i \asp{,J)} : \pi_{3J} \asp{ :- } \textit{CN} : \pi_{3J} \asp{,} C : \pi_{3J} \asp{,}\asp{holdsat(pow(}b\asp{),} \textit{In}^{i}\asp{, I)} : \pi_{3J}, \asp{nifluent(obl(}b, d)\asp{, }\textit{In}^i\asp{)} : \pi_0, \\ \asp{instant(I)} : \pi_{0} \asp{.}$
\item $\text{\ref{eqASPDCATrans2} - } \asp{holdsat(pro(}b, d\asp{)}, \textit{In}^i \asp{,I)} : \pi_{3J} \asp{ :- }$ \\ $\textit{CN}\asp{,} : \pi_{3J} \textit{C} : \pi_{3J} \asp{,} \asp{holdsat(pow(}b\asp{),} \textit{In}^{i}\asp{, I)} : \pi_{3J},$ \\ $\asp{nifluent(pro(}b, d)\asp{, } : \pi_0, \\ \asp{instant(J)} : \pi_{0} \asp{.}$
\item $\text{\ref{eqASPDCATrans5} - } \asp{holdsat(obl(}b, d\asp{)}, \textit{In}^i \asp{,J)} : \pi_{3J} \asp{ :- } \textit{CN} : \pi_{3J} \asp{,} C : \pi_{3J}, \asp{nifluent(obl(}b, d)\asp{, }\textit{In}^i\asp{)} : \pi_0, \\ \asp{instant(I)} : \pi_{0} \asp{.}$
\item $\text{\ref{eqASPDCATrans6} - } \asp{holdsat(pro(}b, d\asp{)}, \textit{In}^i \asp{,I)} : \pi_{3J} \asp{ :- } \textit{CN}\asp{,} : \pi_{3J} \textit{C} : \pi_{3J} \asp{,} \\ \asp{instant(J)} : \pi_{0} \asp{.}$
\item $\text{\ref{eqASPDCATrans3} - } \asp{holdsat(obl(}b, d\asp{)}, \textit{In}^i \asp{,I)} : \pi_{3J} \asp{ :- } \textit{CN}, : \pi_{3J} C  : \pi_{3J} \asp{,} \asp{holdsat(pow(}b\asp{),} \textit{In}^{i}\asp{, I)} : \pi_{3J}, \asp{nifluent(obl(}b, d)\asp{, } \textit{In}^{i} \asp{),}  : \pi_{0}, \asp{instant(I).} : \pi_{0}$
\item $\begin{aligned} \text{\ref{eqASPDCATrans4} - } \asp{holdsat(pro(}b, d\asp{)}, \textit{In}^i \asp{,I)} : \pi_{3J} \asp{ :- } & \textit{CN}, C : \pi_{3J}, \\ & \asp{holdsat(pow(}b\asp{),} \textit{In}^{i}\asp{, I)} : \pi_{3J}, \\ & \asp{nifluent(obl(}b, d)\asp{, } \textit{In}^{i} \asp{),}  : \pi_{0}, \\ & \asp{instant(I).} : \pi_{0} \end{aligned}$
\item $\text{\ref{eqASPCompTraceTrans} -} \asp{observed(\textit{e}_{\textit{i}}, J).} : \pi_{0}$
\item $\begin{aligned} \text{\ref{eqASPSemTrans1} -}
\asp{holdsat(P,In,J)} : \pi_{3J} \asp{:-} & \asp{holdsat(P,In,J)} : \pi_{3J}, \asp{not \; terminated(P,In,H)} : \pi_{3H+2}, \\ &  \asp{next(H,J)} : \pi_{0}  \asp{,} \\ & \asp{ifluent(P, In).} : \pi_{0} \end{aligned}$
\item $\begin{aligned} \text{\ref{eqASPSemTrans2} -}
\asp{holdsat(P,In,J)} : \pi_{3J} \asp{:-} & \asp{initiated(P,In,J)} : \pi_{3J+2}, \\ &
	\asp{next(I,J)} : \pi_{0}, \\ &
    \asp{ifluent(P, In)} : \pi_{0}.
\end{aligned}$
\item $\begin{aligned} \text{\ref{eqASPSemTrans3} -}
\asp{occurred(now, In, J)} : \pi_{3J+1} \asp{:- instant(J)} : \pi_{0}, \asp{inst(In)} : \pi_{0}.
\end{aligned}$
\item $\begin{aligned} \text{\ref{eqASPSemTrans4} -}
\asp{occurred(E,In,J)} : \pi_{3J+1} \asp{:- evtype(E,In,ex)} : \pi_{0} \asp{,observed(E,In,J)}: \pi_{3J}.
\end{aligned}$
\item $\begin{aligned} \text{\ref{eqASPSemTrans5} -}
\asp{occurred(null,In,J)} : \pi_{3J+1} \asp{:- not\; evtype(E,In,ex)} : \pi_{0}, \asp{observed(E,In,J)} : \pi_{3J}.
\end{aligned}$
\item $\begin{aligned} \text{\ref{eqASPSemTrans6} -} \asp{\{observed(E, J)\}} : \pi_{3J} \asp{:-} & \asp{evtype(E,In,ex)} : \pi_{0}, \asp{instant(J)} : \pi_{0}, \asp{not\; final(J)} : \pi_{0}, \\ & \asp{inst(In)} : \pi_{0}. \end{aligned}$
\item $\begin{aligned} \text{\ref{eqASPSemTrans7} -} 
\asp{ :- } & \asp{observed(E,J)} : \pi_{3J},\asp{observed(F,J)} : \pi_{3J}, \asp{instant(J)} : \pi_{0}, \\ & \asp{evtype(E,InX,ex)} : \pi_{0}, \\ & \asp{evtype(F,InY,ex)} : \pi_{0}, E!=F : \pi_{0}, \asp{inst(InX;InY)} : \pi_{0}.
\end{aligned}$
\item $\begin{aligned} \text{\ref{eqASPSemTrans8} -} \asp{obs(J)} : \pi_{3J} \asp{:-} & \asp{observed(E,J)} : \pi_{3J},\asp{evtype(E,In,ex)} : \pi_{0}.
\end{aligned}$
\item $\begin{aligned} \text{\ref{eqASPSemTrans9} -}
\asp{ :- not\; obs(J)} : \pi_{3J}, not\; \asp{final(J)} : \pi_{0}, \asp{instant(J)} : \pi_{0}.
\end{aligned}$
\item $\begin{aligned} \text{\ref{eqASPSemTrans10} -}
\asp{observed(E,In,J)} : \pi_{3J} :- \asp{observed(E,J)} : \pi_{3J}, \asp{inst(In)} : \pi_{0}.
\end{aligned}$
\item $\begin{aligned} \text{\ref{eqASPSemTrans11} -}
\asp{occurred(disch(obl(A, D)),In,J)} : \pi_{3J+1} \asp{:-} & \asp{holdsat(obl(A, D),In,J)} : \pi_{3J} , \\
& \asp{1\{occurred(A,In,J)} : \pi_{3J+1}, \\ & \asp{holdsat(A, In, J)} : \pi_{3J} \asp{\}.}
\end{aligned}$
\item $\begin{aligned} \text{\ref{eqASPSemTrans12} -} \asp{occurred(viol(obl(a, d))},\textit{In}^{i}, \asp{J)} : \pi_{3J+1} \asp{:-} & \asp{holdsat(obl(a, d)},\textit{In}^{i}, \asp{J)} : \pi_{3J} \asp{,} \\ & \asp{not\;} \\ & \asp{occurred(} \\ & \asp{disch(obl(a, d))}, \textit{In}^{i}, \asp{J)} : \pi_{3J+1} \asp{,} \\ & 
\asp{1\{occurred(d},\textit{In}^{i}, \asp{J)} : \pi_{3J+1} \asp{,} \\ & 
\asp{holdsat(d,} \textit{In}^{i}, \asp{J)\} } : \pi_{3J} \asp{.} \end{aligned}$.
\item $\begin{aligned}\text{\ref{eqASPSemTrans13} -}\asp{occurred(disch(pro(A, D)),In,J)} : \pi_{3J+1} \asp{:-} & \asp{
   holdsat(pro(A, D),In,J)} : \pi_{3J}, \\ & 
   \asp{1\{occurred(D,In,J),} : \pi_{3J+1} \\ & \asp{holdsat(D, In, J)} : \pi_{3J} \asp{\}.} \end{aligned}$
\item $\begin{aligned}\text{\ref{eqASPSemTrans14} -}
\asp{occurred(viol(pro(A, D)),In,J)} : \pi_{3J+1} \asp{:-} & \asp{holdsat(pro(A, D)),In,J)}: \pi_{3J} \asp{,} \\ & \asp{1\{occurred(A,In,J)} : \pi_{3J+1} \asp{,} \\ & 
\asp{holdsat(A, In, J)} : \pi_{3J} \asp{\}}, \\ & \asp{not\; occurred(} \\ & \asp{disch(pro(A, D)), In, J)} : \pi_{3J+1}.\end{aligned}$
\item $\begin{aligned} \text{\ref{eqASPSemTrans15} -}
\asp{terminated(N,In,J)} : \pi_{3J+2} \asp{:-} &
   \asp{1\{occurred(viol(N),In,J)} : \pi_{3J+1}, \\ & \asp{occurred(disch(N),In,J)} : \pi_{3J+1} \asp{\}}, \\& \asp{ifluent(N,In)} : \pi_{0}, \asp{holdsat(N,In,J) : \pi_{3J}.}
\end{aligned}$
\item $\begin{aligned} \text{\ref{eqASPSemTrans16} -} & \asp{final(\textit{k})} : \pi_{0} .\; \\ &
 \asp{start(0)} : \pi_{0}. \; \asp{instant(0..T) : \pi_{0} :- final(T)}: \pi_{0}.  \; \\ &
 \asp{next(T, T+1)} : \pi_{0} \asp{:- instant(T)} : \pi_{0} . \end{aligned}$
% Note for future in case needed: Initially I was going to prove that we do not have a cyclic dependency graph by the fact that M_P is a model (in the formal framework). However, since we are only dealing with applied rules this is not necessary. We also do not need to prove that P is in general stratisfied (which isn't true). Since there is not always a unique answer-set, there is no answer-set if there is no model in the formal framework due to an ontological inconsistency.
\end{itemize}
Now we will show $M_P$ is a minimal model. Let $Z$ be an interpretation such that $Z \subset M_P$. Let $l$ be the lowest strata in which $Z$ and $M_P$ differ in atoms for $P^{*, M_P, \prime}$. Let $S$ be the set of atoms $s \in S$ such that $s : \pi_l$ is stratified at strata $l$ and $s \in M_P \backslash Z$. For an $s \in S$ we show it must be the head of an applied rule in $P^{*, M_P \prime}$.
\begin{enumerate}[label*=\arabic*.]
\item $s$ is a fact, then $Z$ cannot be a model of $P^{*, M_P \prime}$ since one of \ref{eqASPMLTrans1}-\ref{eqASPMLTrans5} or a fact in \ref{eqASPSemTrans16} is not applied.
\item $s = \asp{holdsat(}f^{\prime}, \textit{In}^{i}, j)$ -
\begin{enumerate}[label*=\arabic*.]
\item By $M_P \models s$ and construction we have $S^{i}_{j} \models f^{\prime}$, therefore either:
\begin{enumerate}[label*=\arabic*.]
\item by Definition~\ref{defStateForm} and construction of $M_P$: $M_P \models \asp{holdsat}(f, \textit{In}^{i}, j)$ for a rule $r$ created by \ref{eqASPMLTrans11}, or
\item by Definition~\ref{eqIS1} \ref{eqIS2} and construction of $M_P$: $M_P \models \asp{holdsat}(f, \textit{In}^{i}, j)$ for a rule $r$ created by \ref{eqASPMLTrans10}, or
\item by Definition~\ref{defDC} and construction of $M_P$: $M_P \models \textit{EX}(X, \pazocal{I}^{i})$, in the case of \ref{eqDCCl2} $M_P \models \asp{holdsat}(\textit{pow}(b, \textit{In}^{i}, j)$ and $M_P \models \textit{EX}(N, \pazocal{I}^{i})$ for a rule $r$ created by \ref{eqASPDCATrans1}, \ref{eqASPDCATrans2}, \ref{eqASPDCATrans5}, \ref{eqASPDCATrans6}, \ref{eqASPDCATrans3}, \ref{eqASPDCATrans4}, or 
\item by Definition~\ref{defST} or by Definition~\ref{defInitialStates} and construction of $M_P$: $M_P \models \textit{EX}(X, \pazocal{I}^{i})$ and $M_P \models \textit{EX}(X, \pazocal{I}^{i})$ and $M_P \models \asp{holdsat}(g, \textit{In}^{i}, j)$ for a rule $r$ created by \ref{eqASPMLTrans13}, or
\item by \ref{eqST11} $M_P \models \asp{holdsat}(f, \textit{In}^{i}, j-1)$ for the rule $r$ \ref{eqASPSemTrans1}, or 
\item by \ref{eqST12} and construction of $M_P$: $M_P \models \asp{initiated}(f, \textit{In}^{i}, j)$ for the rule $r$ \ref{eqASPSemTrans2}.
\end{enumerate}
For each possible $r$ the atoms true in the body of the rule are of a lower strata to $s$ and therefore must be in $Z$. Thus, one of the rules is applicable but not applied. Thus $Z$ cannot be a model.
\end{enumerate}
\item $s = \asp{occurred}(e, \textit{In}^{i}, j)$ - by construction $M_P \models s$ means that $e \in E^{i}_{j}$, implying $e \in \pazocal{E}^{i}$. We deal separately with each type of event in $\pazocal{E}$:
\begin{enumerate}[label*=\arabic*.]
\item $e \in \pazocal{E}^{i}_{\textit{obs}}$ - by construction of $M_P$ this implies $\asp{observed}(e, j). \in P^{*}$, a fact, therefore either $Z \not \models \asp{observed}(e, j)$ and $Z$ is not a model, or $Z \models \asp{observed}(e, j)$ meaning \ref{eqASPSemTrans4} is applied and thus for $Z$ to be a model we must have $Z \models \asp{occurred}(e, \textit{In}^{i}, j)$ but we do not and thus $Z$ is not a model.
\item $e \in \pazocal{E}^{i}_{\textit{inst}}$ - by construction of $M_P$ this implies either condition \ref{eqGR13} or \ref{eqGR18} for $e \in E^{i}_{j}$ are true. Respectively, we must have a rule $r \in P^{*}$ of type \ref{eqASPMLTrans9} or \ref{eqASPMLTrans14} such that $H(r) = \asp{occurred}(e, \textit{In}^{i}, j)$. The rule $r$ has body literals of a lower strata than $s$ thus they must be modelled by $Z$, this means $r$ is applied and therefore since $Z \not \models s$ thus $Z$ is not a model.
\item $e = e_{\textit{null}}$ - by \ref{eqThCo7} this implies $e_{\textit{null}} = \textit{str}^{i}_{j}$ therefore by the definition of a synchronised trace, Definition~\ref{defSynchTrace}, we have a composite event trace $\langle \textit{ctr}_0, ..., \textit{ctr}_{k} \rangle$ such that $\textit{ctr}_j \not \in \pazocal{E}_{\textit{obs}}$. This implies we do not have a fact $\asp{evtype}(\textit{ctr}_j, \textit{In}^{i}, \asp{ex)}. \in P^{*}$ by \ref{eqASPMLTrans2}. Therefore, by the reduct we have an applicable rule $r \in P^{*}$ of the type \ref{eqASPSemTrans5} such that $H(r) = \asp{occurred(null}\textit{In}^{i}, j \asp{)}$. However, since $Z \not \models \asp{occurred(null}\textit{In}^{i}, j \asp{)}$ then $r$ is not applied, meaning $Z$ is not a model.
\item $e \in \pazocal{E}^{i}_{\textit{norm}}$ - this implies the conditions of one of \ref{eqGR14}, \ref{eqGR15}, \ref{eqGR16} must be true \ref{eqGR17}. Thus, by construction of $E^{i}_{j}$ and $S^{i}_{j}$ we have the conditions for a rule $r$ of type \ref{eqASPSemTrans11}, \ref{eqASPSemTrans12}, \ref{eqASPSemTrans13} or \ref{eqASPSemTrans14} such that $H(r) = \asp{occurred}(e, \textit{In}^{i}, j)$. Since by the reduct negated elements of $B(r)$ are removed, all remaining elements of $B(r)$ are of a lower strata than $s$ therefore all body elements of $r$ are true and thus $r$ is an applicable rule. However, since $Z \not \models \asp{occurred}(e, \textit{In}^{i}, j)$ we know $r$ is not applied and therefore $Z$ is not a model.
\end{enumerate}
\item $s = \asp{initiated}(f, \textit{In}^{i}, j)$ - by \ref{eqThCo4} we know that $f \in S^{i}_{j}$, $f \not \in S^{i}_{j-1}$ and $f \in \pazocal{F}^{i}_{\textit{inert}}$. Since $M$ is a model this means we must have by Definition~\ref{defIndFlInTe} $f \in \textit{INIT}(S^{i}_{j}, E^{i}_{j})$:
\begin{enumerate}[label*=\arabic*.]
\item Condition \ref{eqFIT11} - thus we have $S^{i}_{j} \models f$, $f \in \pazocal{C}^{i \uparrow}(X, e)$, $S^{i}_{j} \models X$ and $e \in E^{i}_{j}$. By the creation of $E^{i}_{j}$ and $S^{i}_{j}$ this means we have all the conditions for an applicable rule $r \in P^{*}$ of type \ref{eqASPMLTrans6} such that $H(r) = s$ and all the body literals are true in $M_P$. Since all the body literals are of a lower strata than $s$ we conclude they are also true in $Z$, therefore $r$ is an applicable rule but since $Z \not \models s$ it is not applied and therefore $Z$ is not a model.
\end{enumerate}
\item $s = \asp{terminated}(f, \textit{In}^{i}, j)$ - by \ref{eqThCo4} we know that $f \in S^{i}_{j}$, $f \not \in S^{i}_{j+1}$ and $f \in \pazocal{F}^{i}_{\textit{inert}}$. Since $M$ is a model this means we must have by Definition~\ref{defIndFlInTe} $f \in \textit{TERM}(S^{i}_{j}, E^{i}_{j})$. We deal with each of the conditions required for $f$ to be in one of these sets:
\begin{enumerate}[label*=\arabic*.]
\item Condition \ref{eqFIT21} - thus we have $S^{i}_{j} \models f$, $f \in \pazocal{C}^{i \downarrow}(X, e)$, $S^{i}_{j} \models X$ and $e \in E^{i}_{j}$. By the creation of $E^{i}_{j}$ and $S^{i}_{j}$ this means we have all the conditions for an applicable rule $r \in P^{*}$ of type \ref{eqASPMLTrans7} such that $H(r) = s$ and all the body literals are true in $M_P$. Since all the body literals are of a lower strata than $s$ we conclude they are also true in $Z$, therefore $r$ is an applicable rule but since $Z \not \models s$ it is not applied and therefore $Z$ is not a model.
\item Condition \ref{eqFIT22} - thus we have $S^{i}_{j} \models f$, and $\textit{viol}(f) \in E^{i}_{j}$ or $\textit{disch}(f) \in E^{i}_{j}$. Since $f \in \pazocal{F}^{i}_{\textit{inert}}$ we have by \ref{eqASPMLTrans4} $\asp{ifluent}(f, \textit{In}^{i})\asp{.} \in P^{*}$ is a fact. By the creation of $E^{i}_{j}$ and $S^{i}_{j}$ this means we have all the conditions for an applicable rule $r \in P^{*}$ of type \ref{eqASPSemTrans15} such that $H(r) = s$ and all the body literals are true in $M_P$. Since all the body literals are of a lower strata than $s$ we conclude they are also true in $Z$, therefore $r$ is an applicable rule but since $Z \not \models s$ it is not applied and therefore $Z$ is not a model.
\end{enumerate}
\item $s = \asp{next}(j, j+1)$ - by \ref{eqThCo15} this implies $j < k$ thus by the rule $\ref{eqASPSemTrans16}$ with the $\asp{instant/3}$ atom in the head we have $M_P \models \asp{instant(}j)$. Thus we have an applicable rule $r \in P^{*}$ where $H(r) = \asp{next}(j, j+1)$ of type at \ref{eqASPSemTrans16} with a body atom that is true in $M_P$. Since the body comprises only an $\asp{instant/3}$ atom of a lower strata than $s$ it is also true in $Z$. But since $Z \not \models s$ it is not applied and therefore $Z$ is not a model.
\end{enumerate}
Therefore, we have shown for all possible cases that $Z$ cannot be a model if it is a strict subset of $M_P$ differing on strata $i$. Thus, $M_P$ is a \textit{minimal model} of $P^{*,M_P}$ and therefore an answer-set for $P^{*}$.
\end{proof}
